# Supplementary material for: On the coupling of magnetic moments to superconducting quantum interference devices
Source: arXiv:2307.05724 source file (2023-07-11)

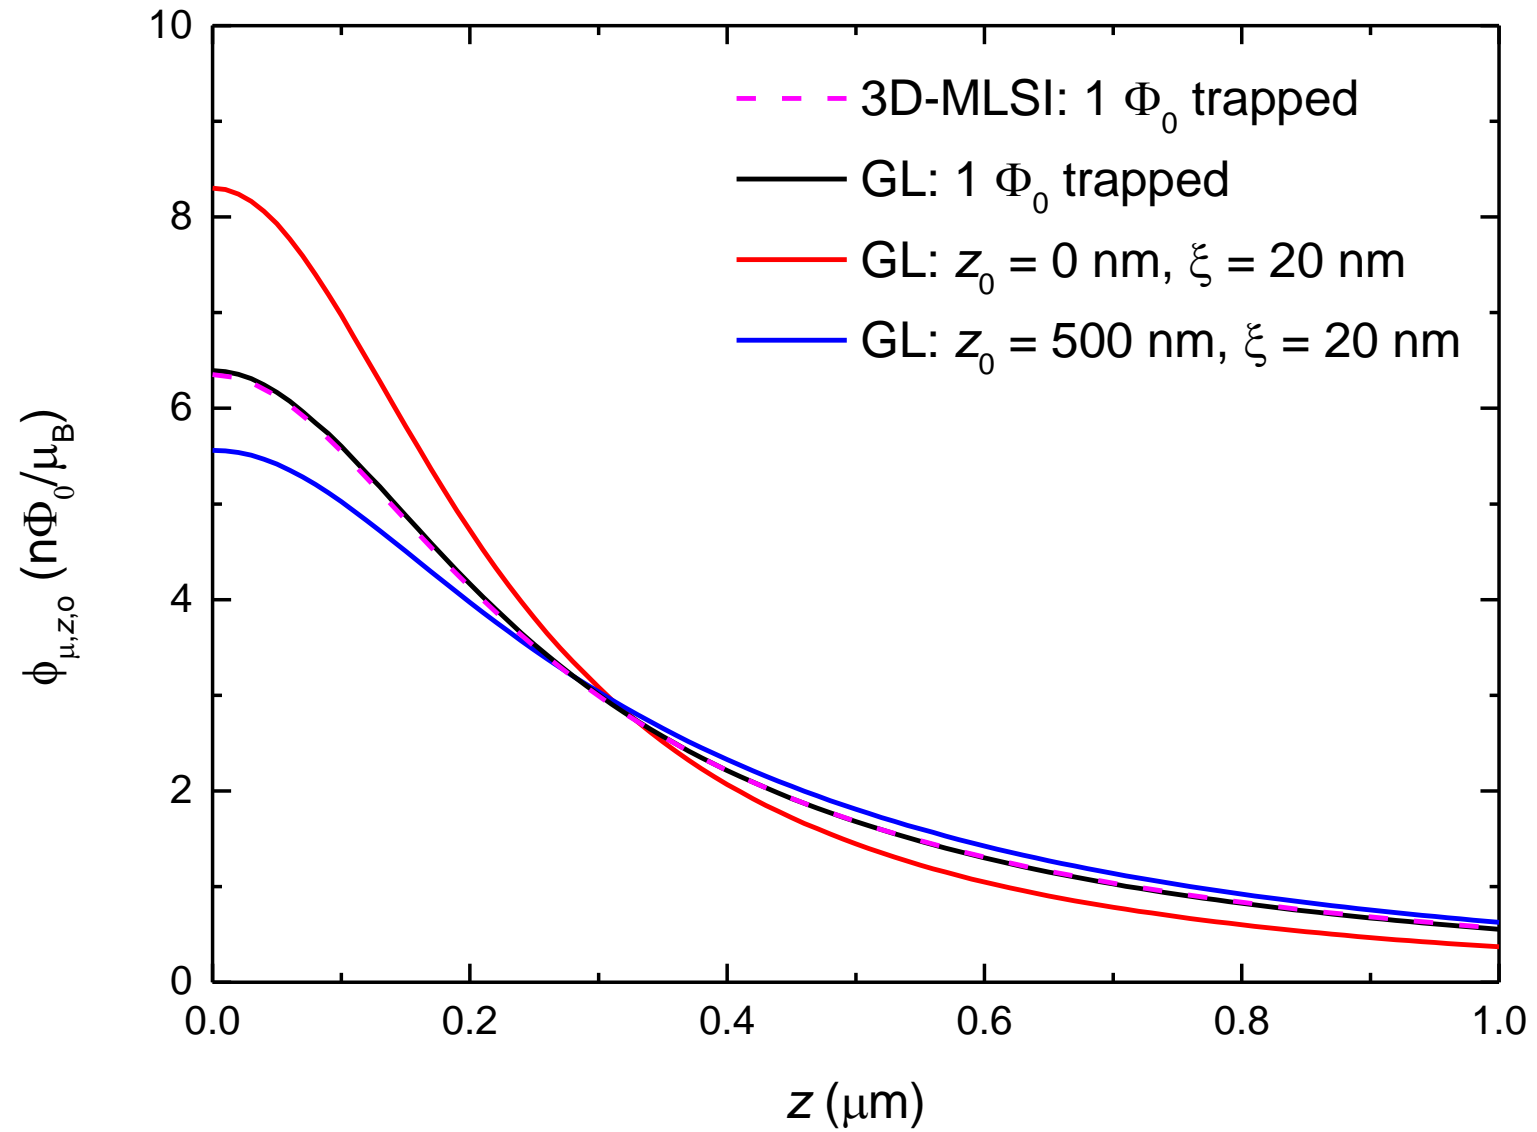

Fig:far\_field\_bigger\_loop\_comparison

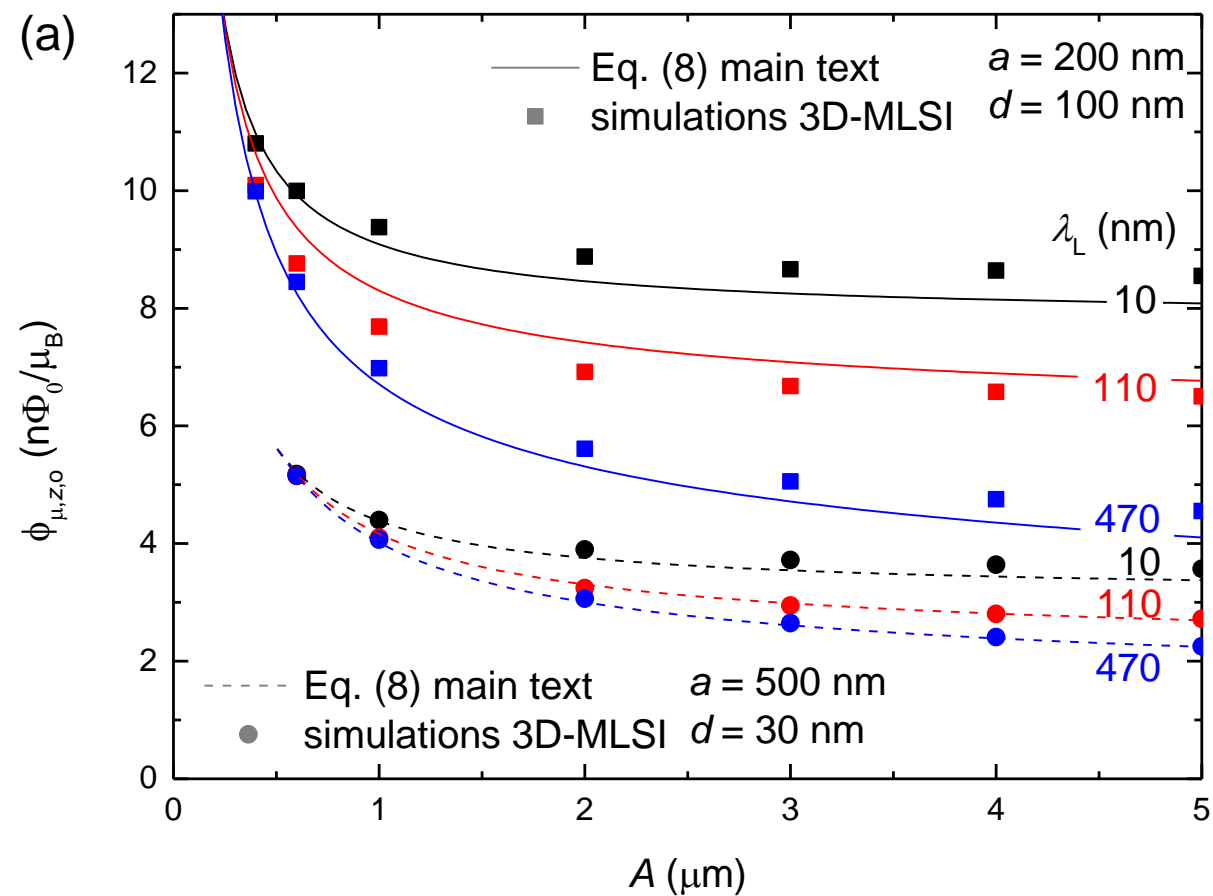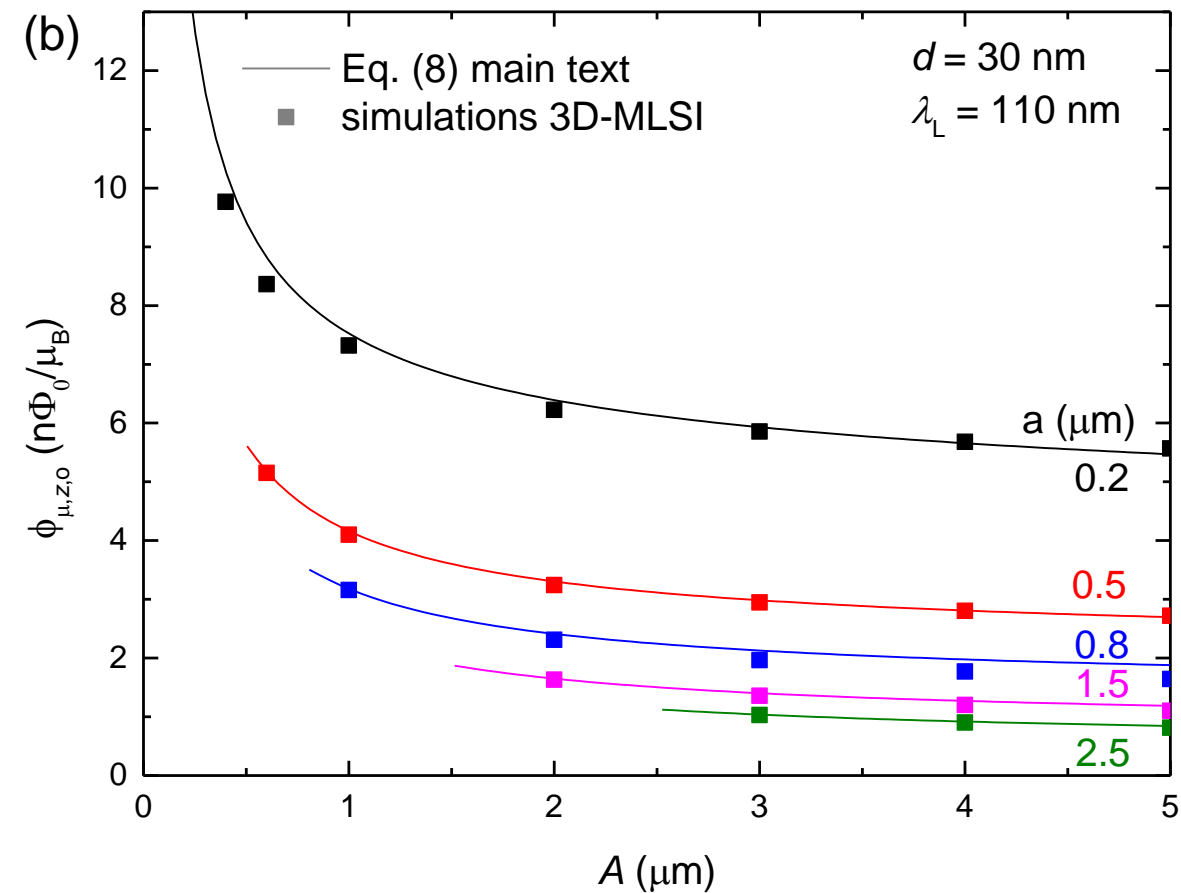

Fig:circ\_A

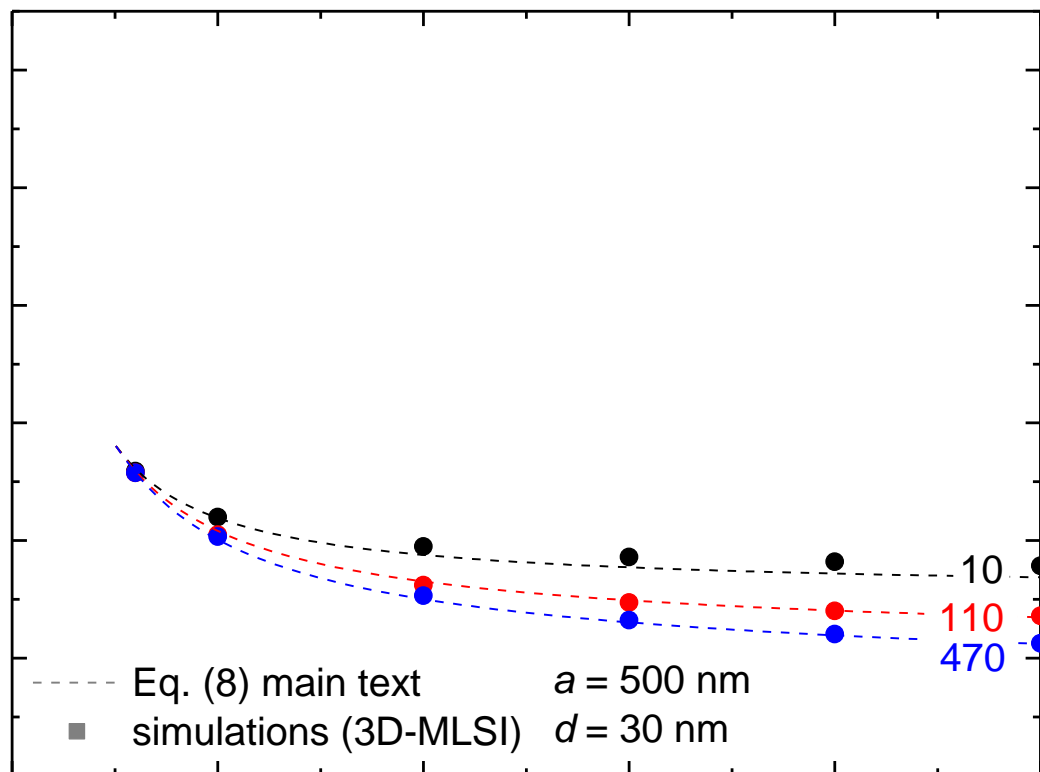

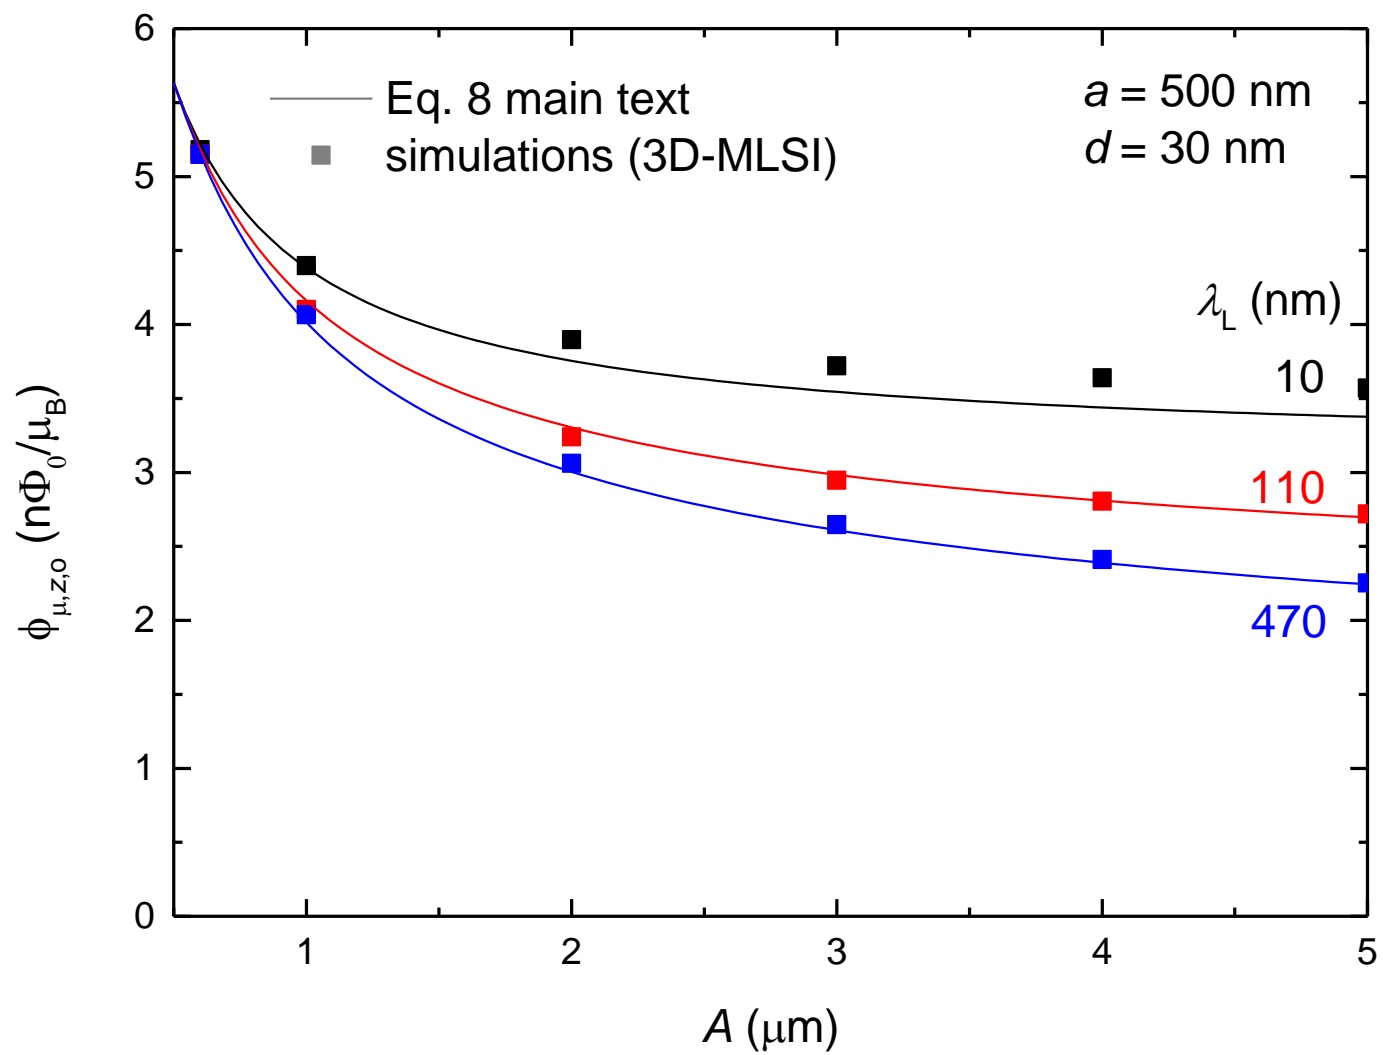

Fig:circ\_a\_500

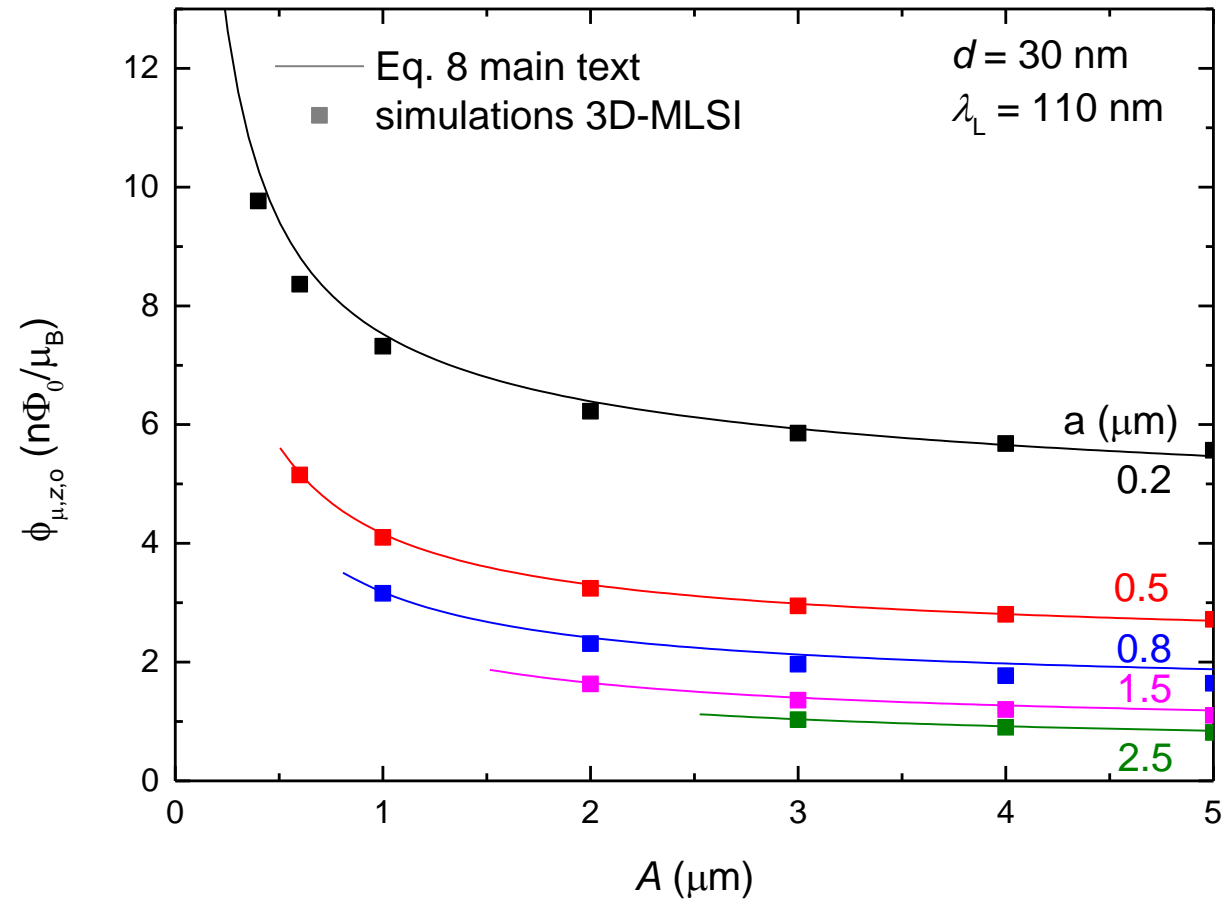

Fig:circ\_a\_var

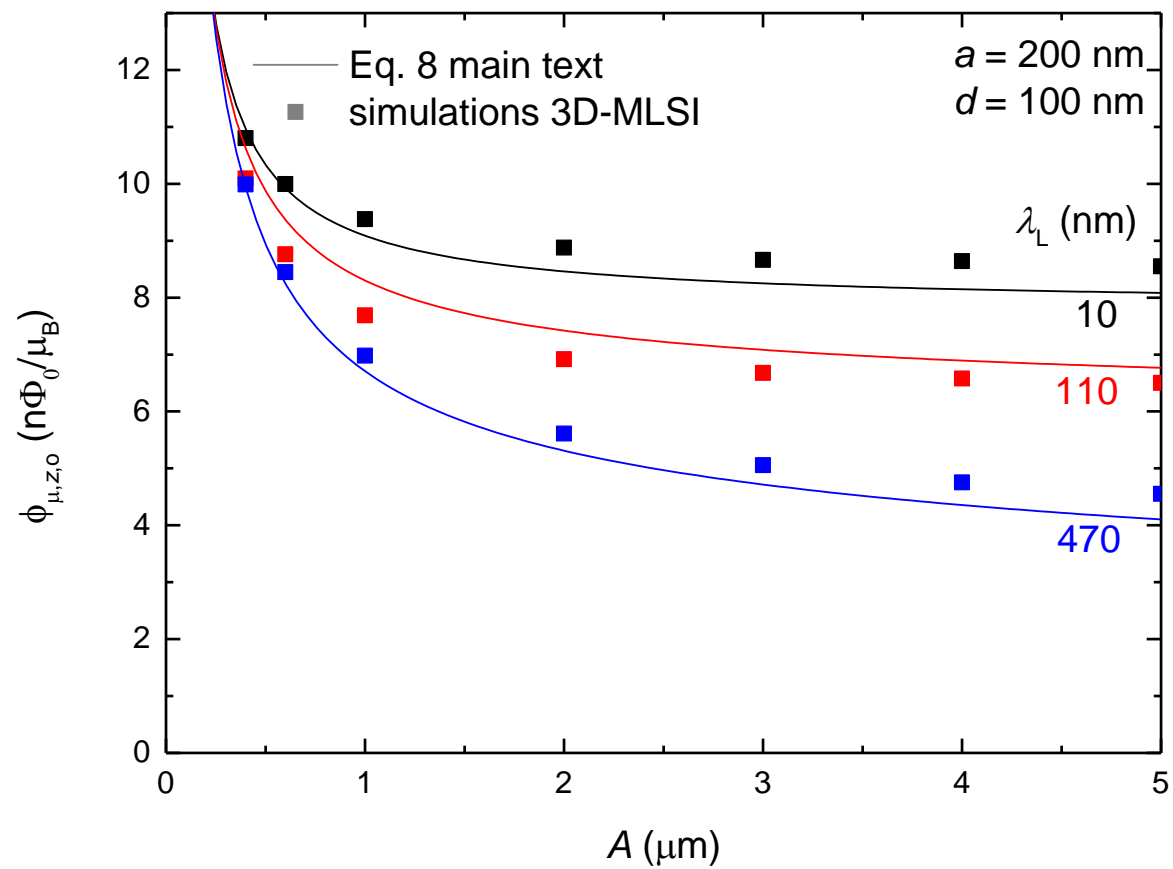

Fig:circ\_a\_200

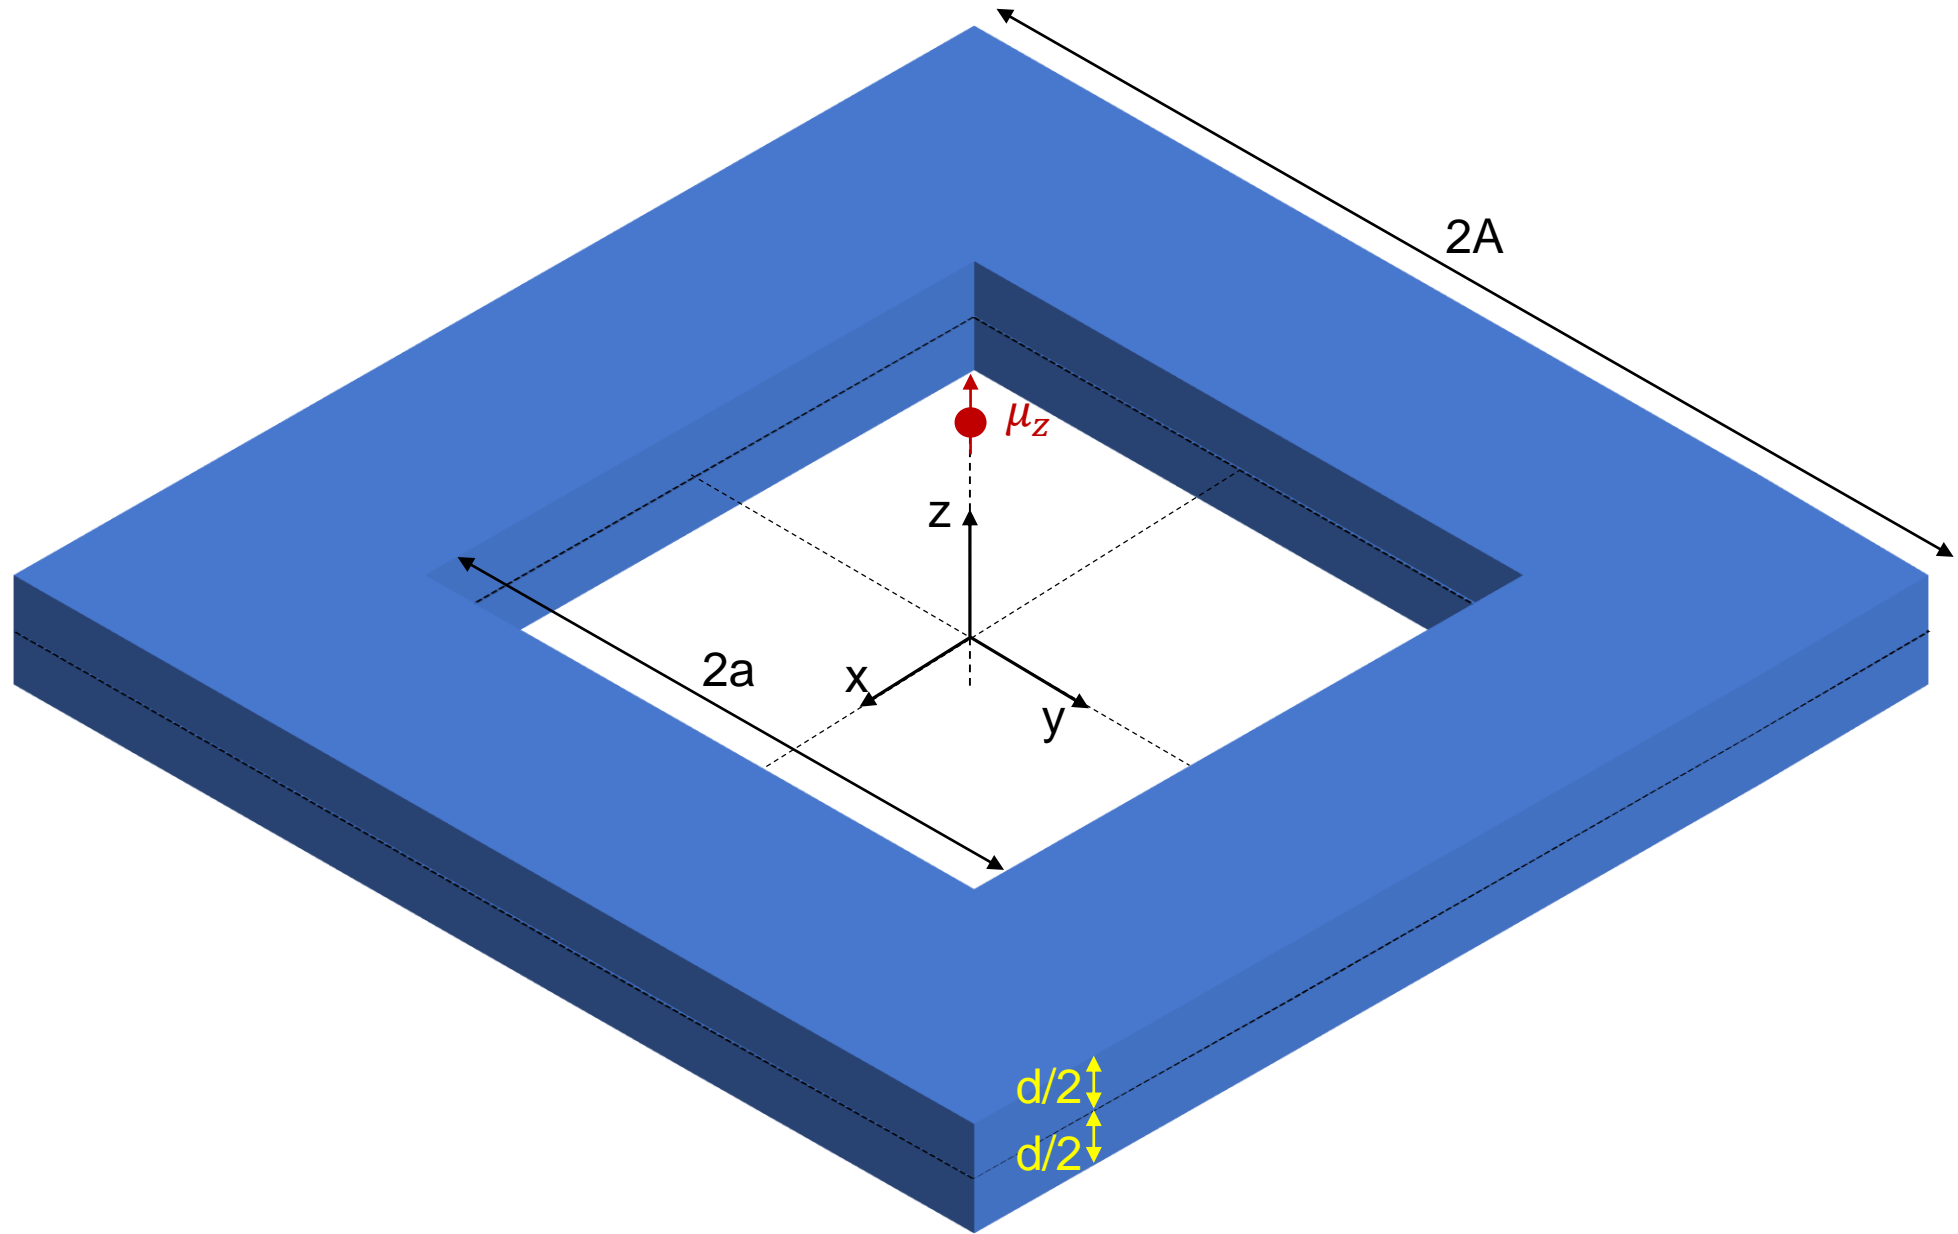

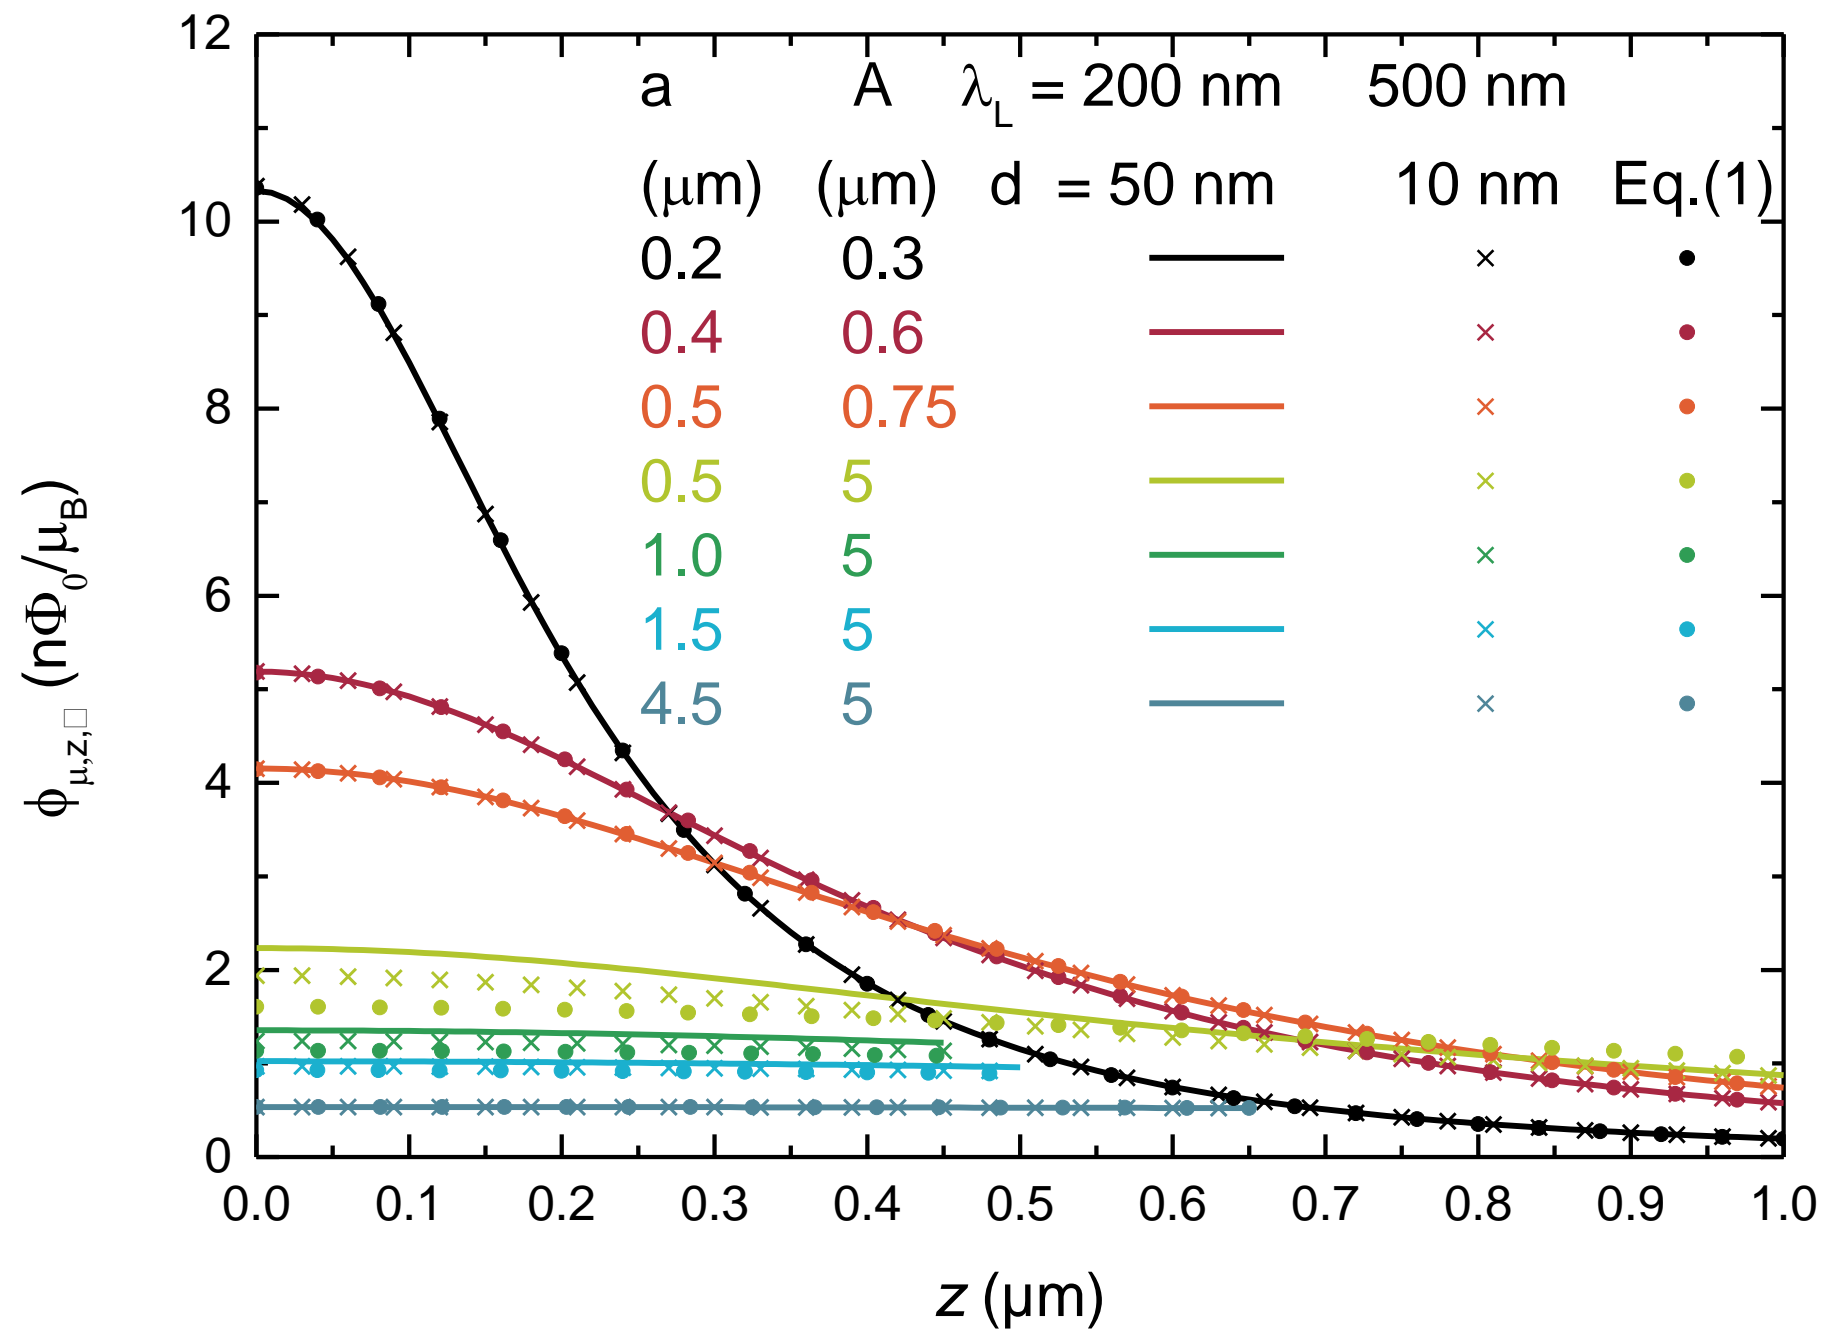



Altes Delta 1.15

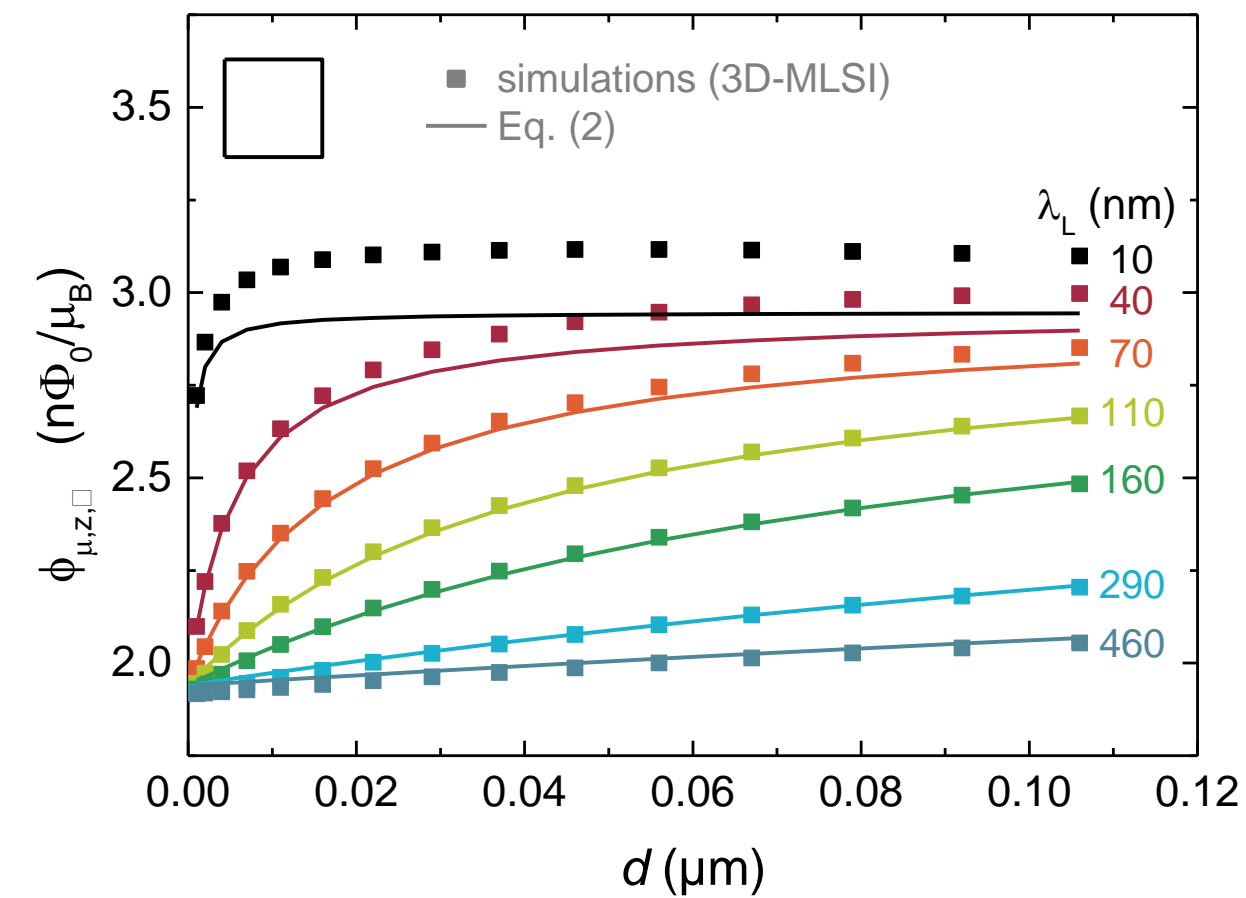

Neues Delta 1.11

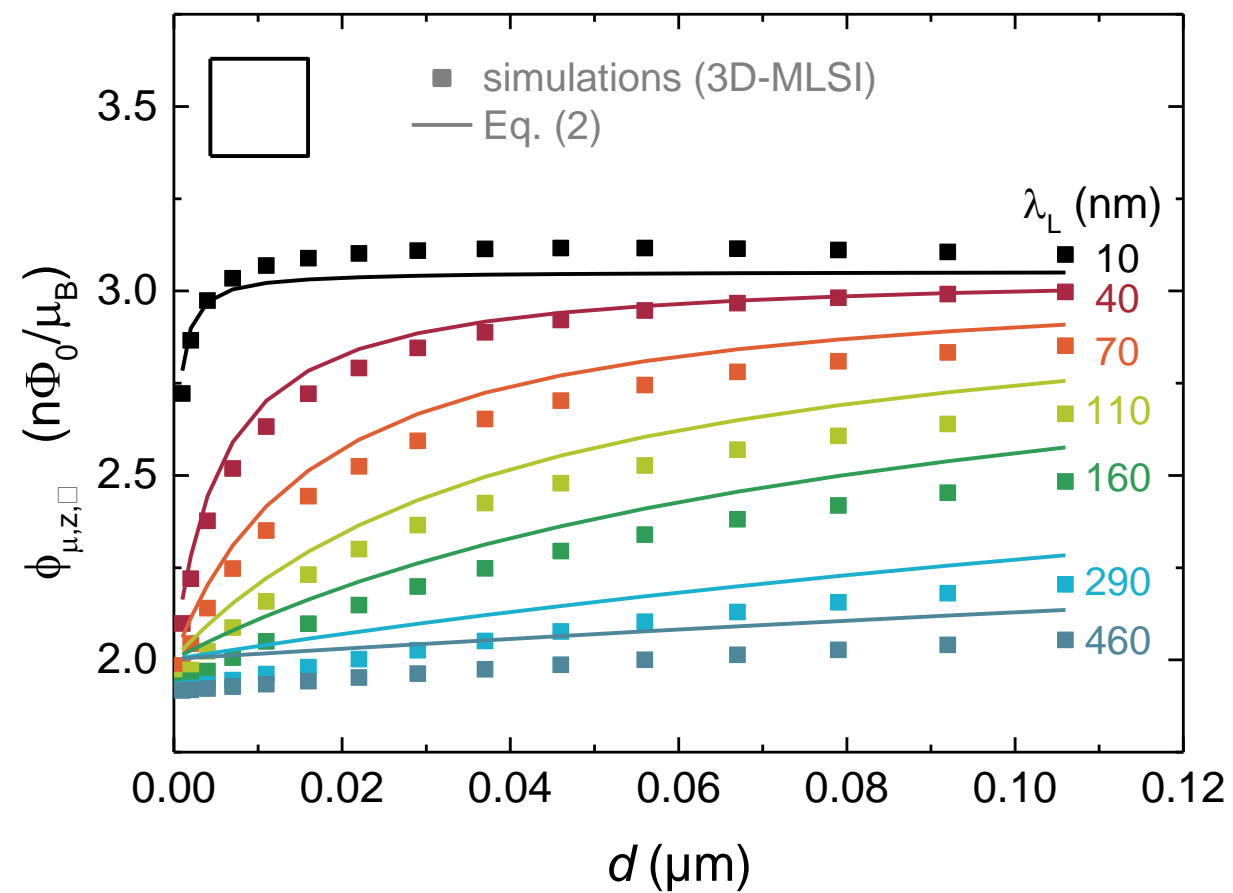

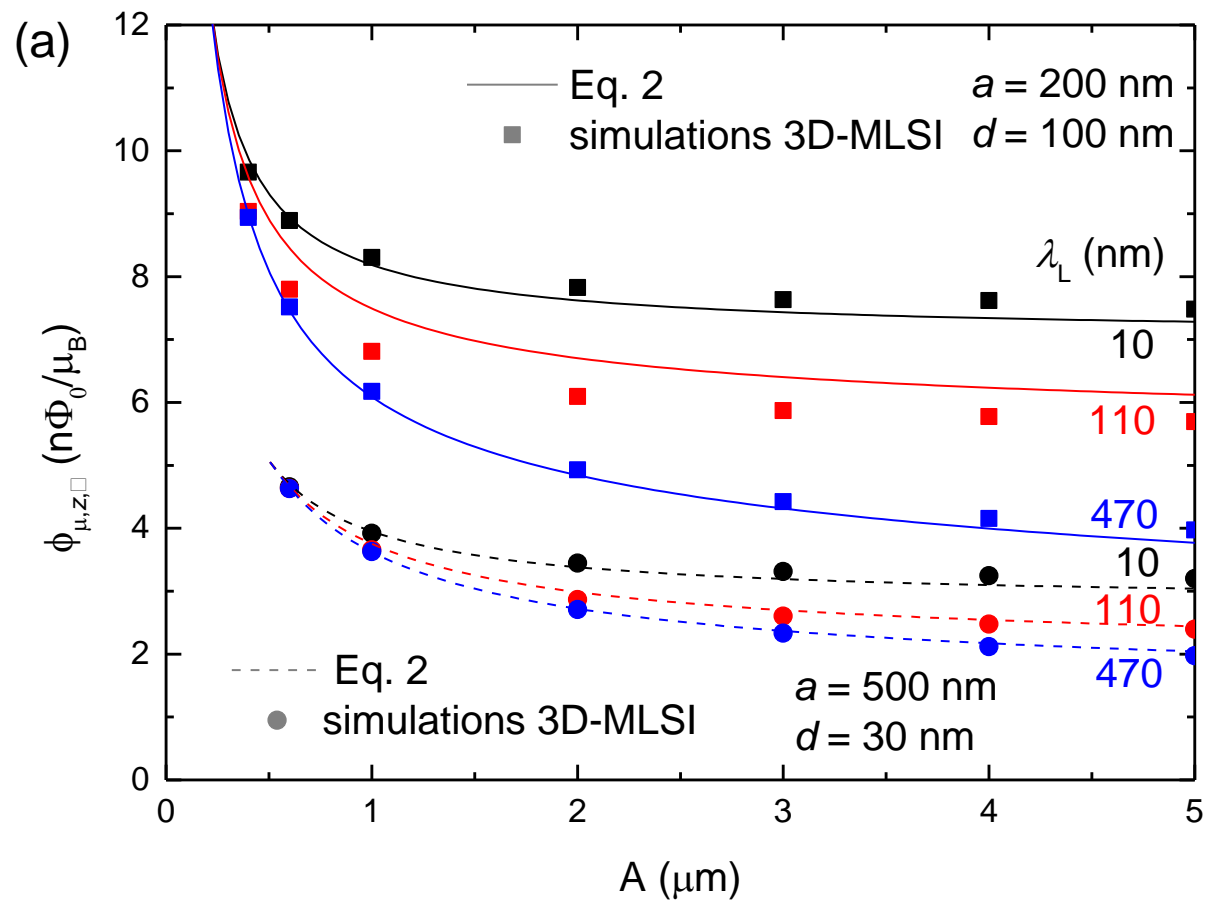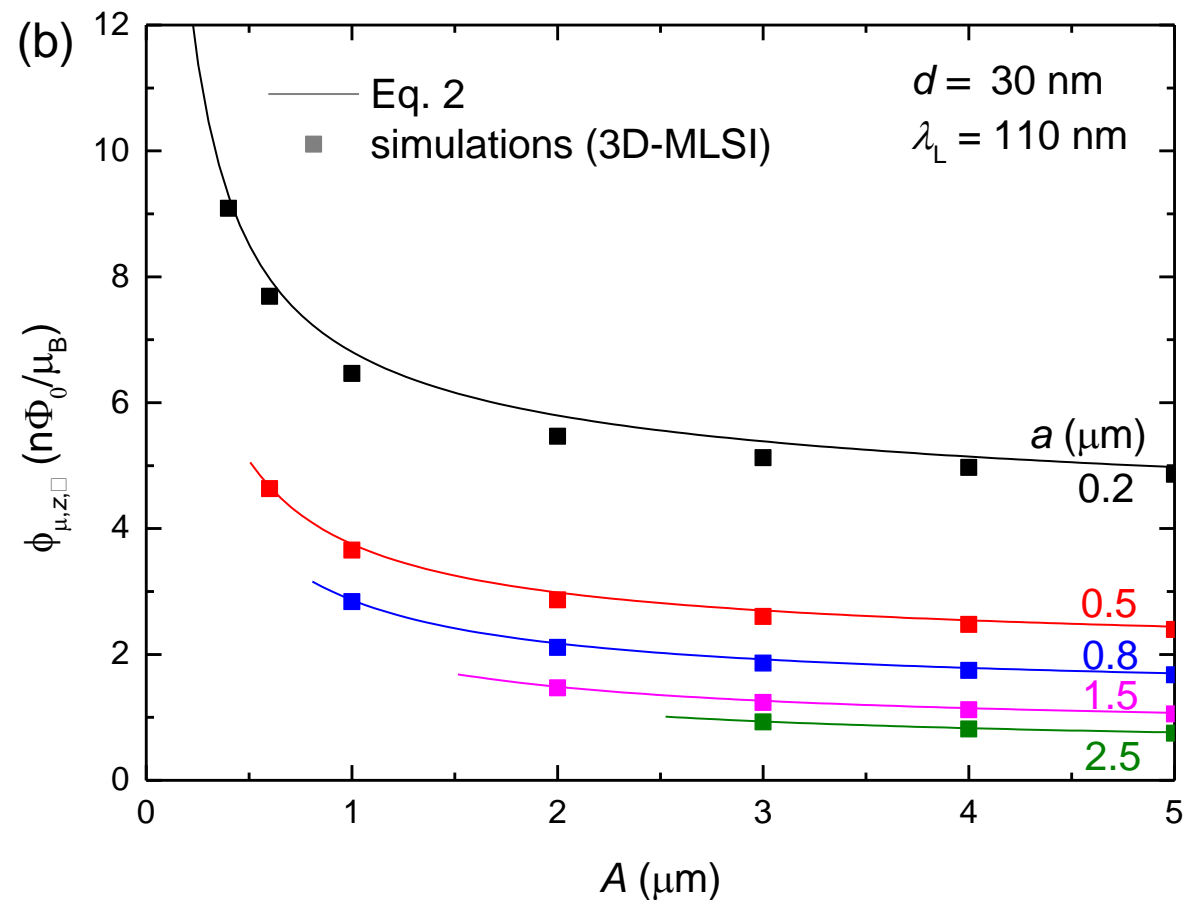

Fig:square\_A

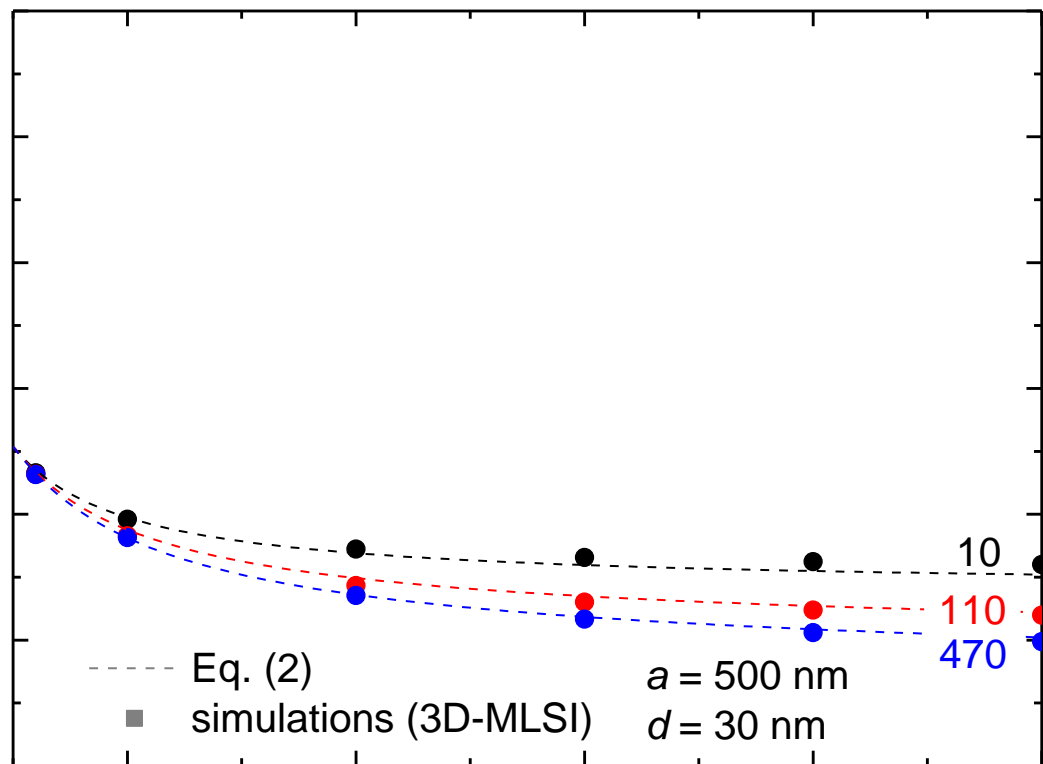

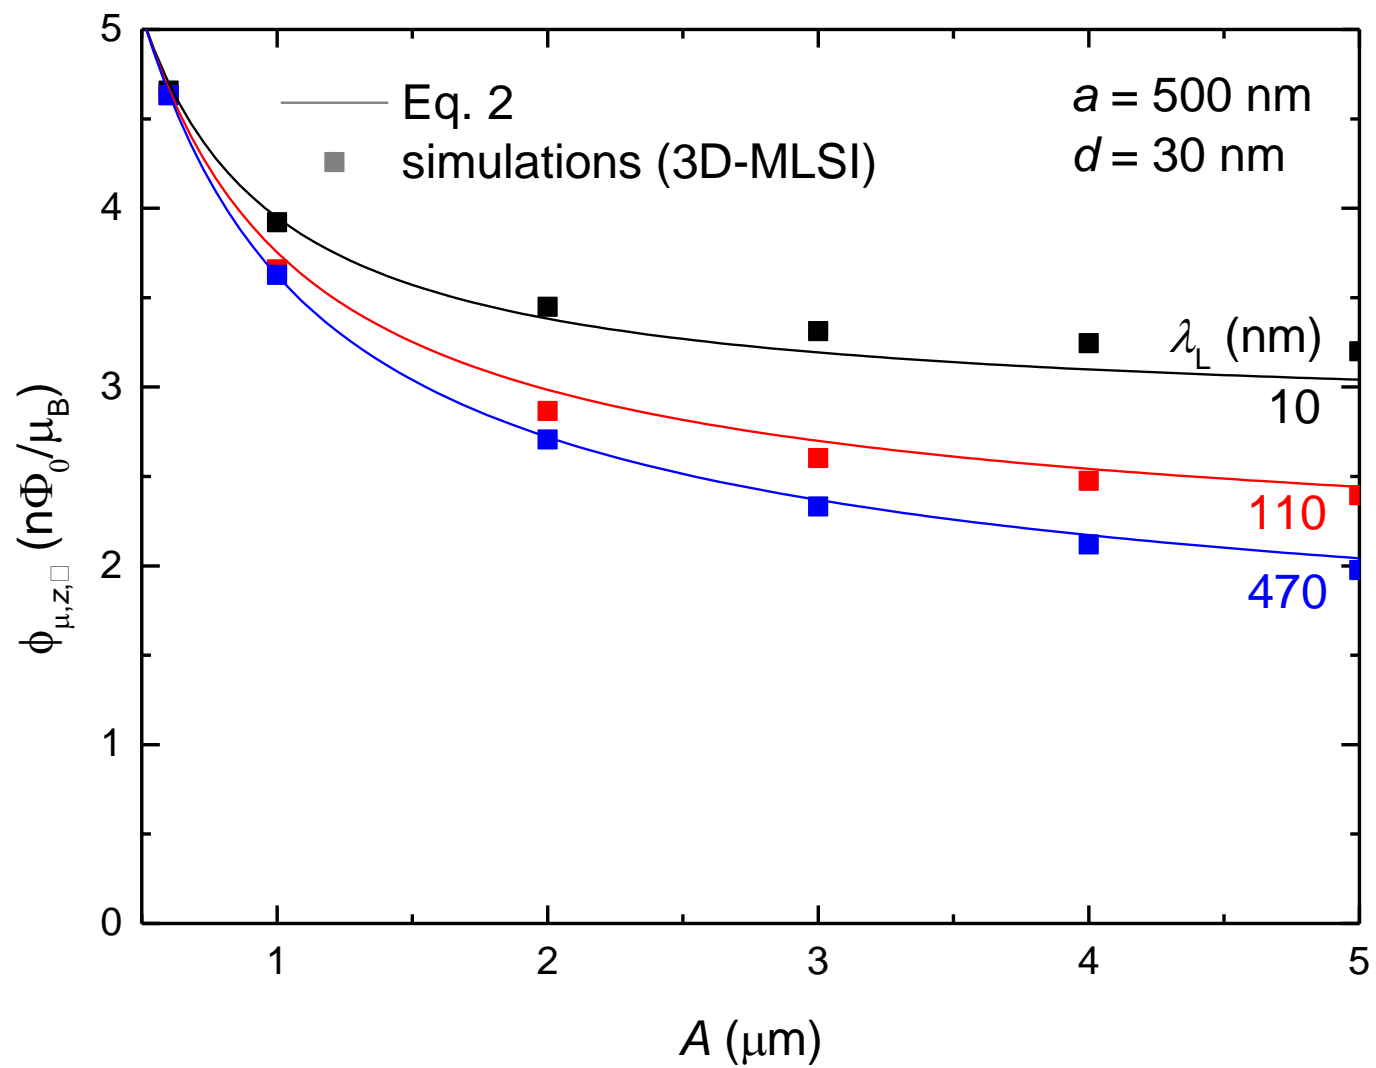

Fig:square\_a\_500

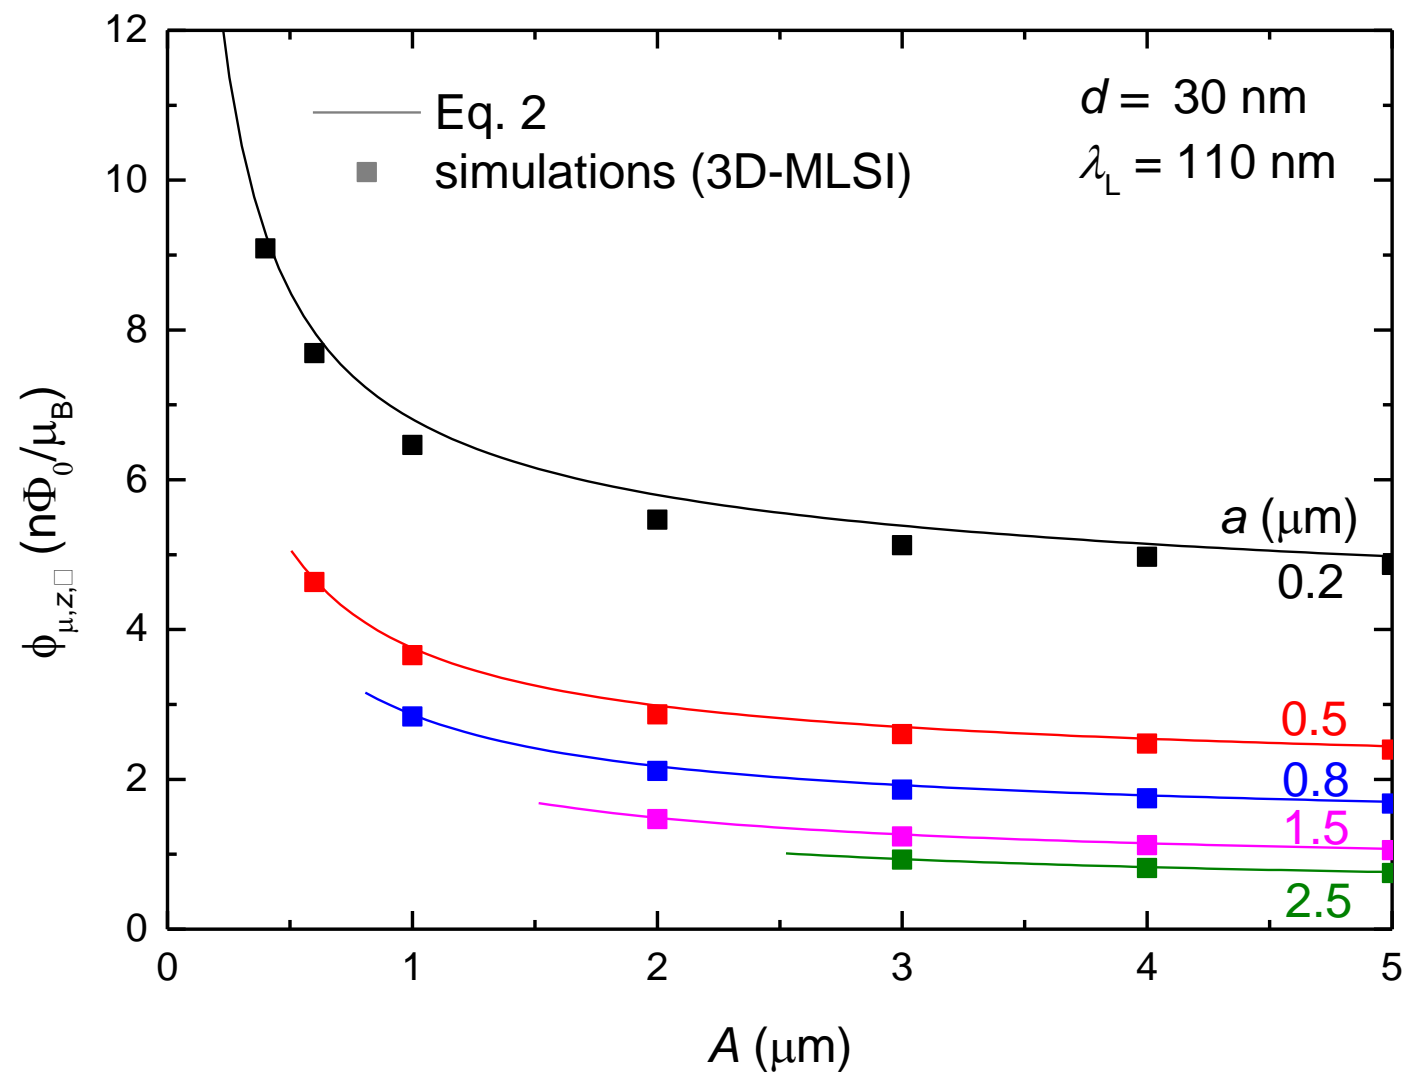

Fig:square\_a\_var

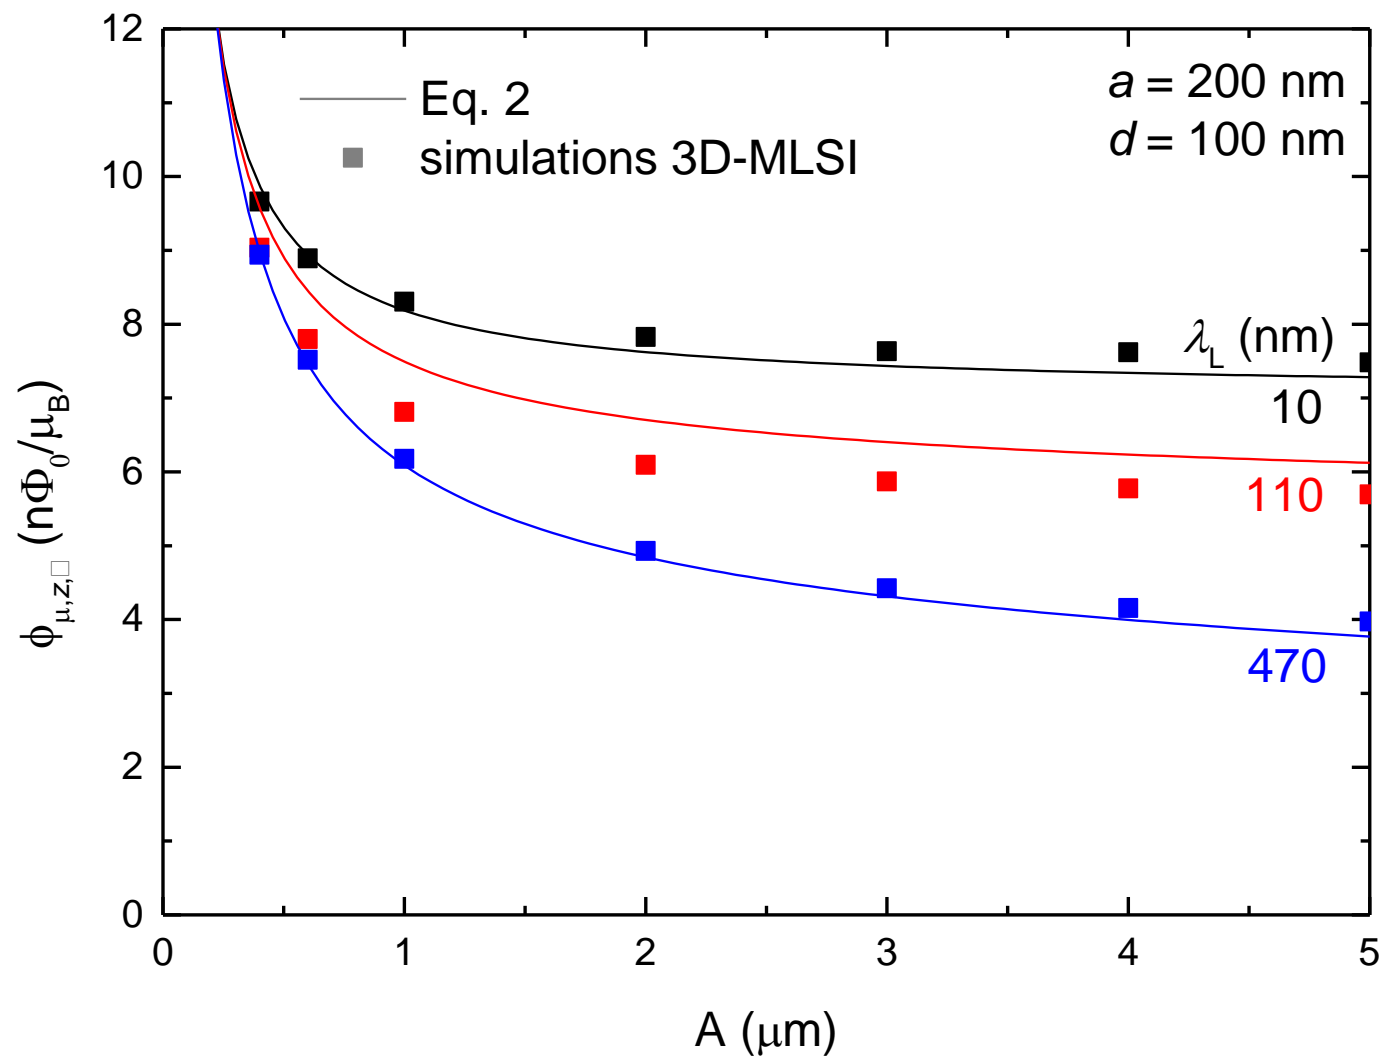

Fig:square\_a\_200

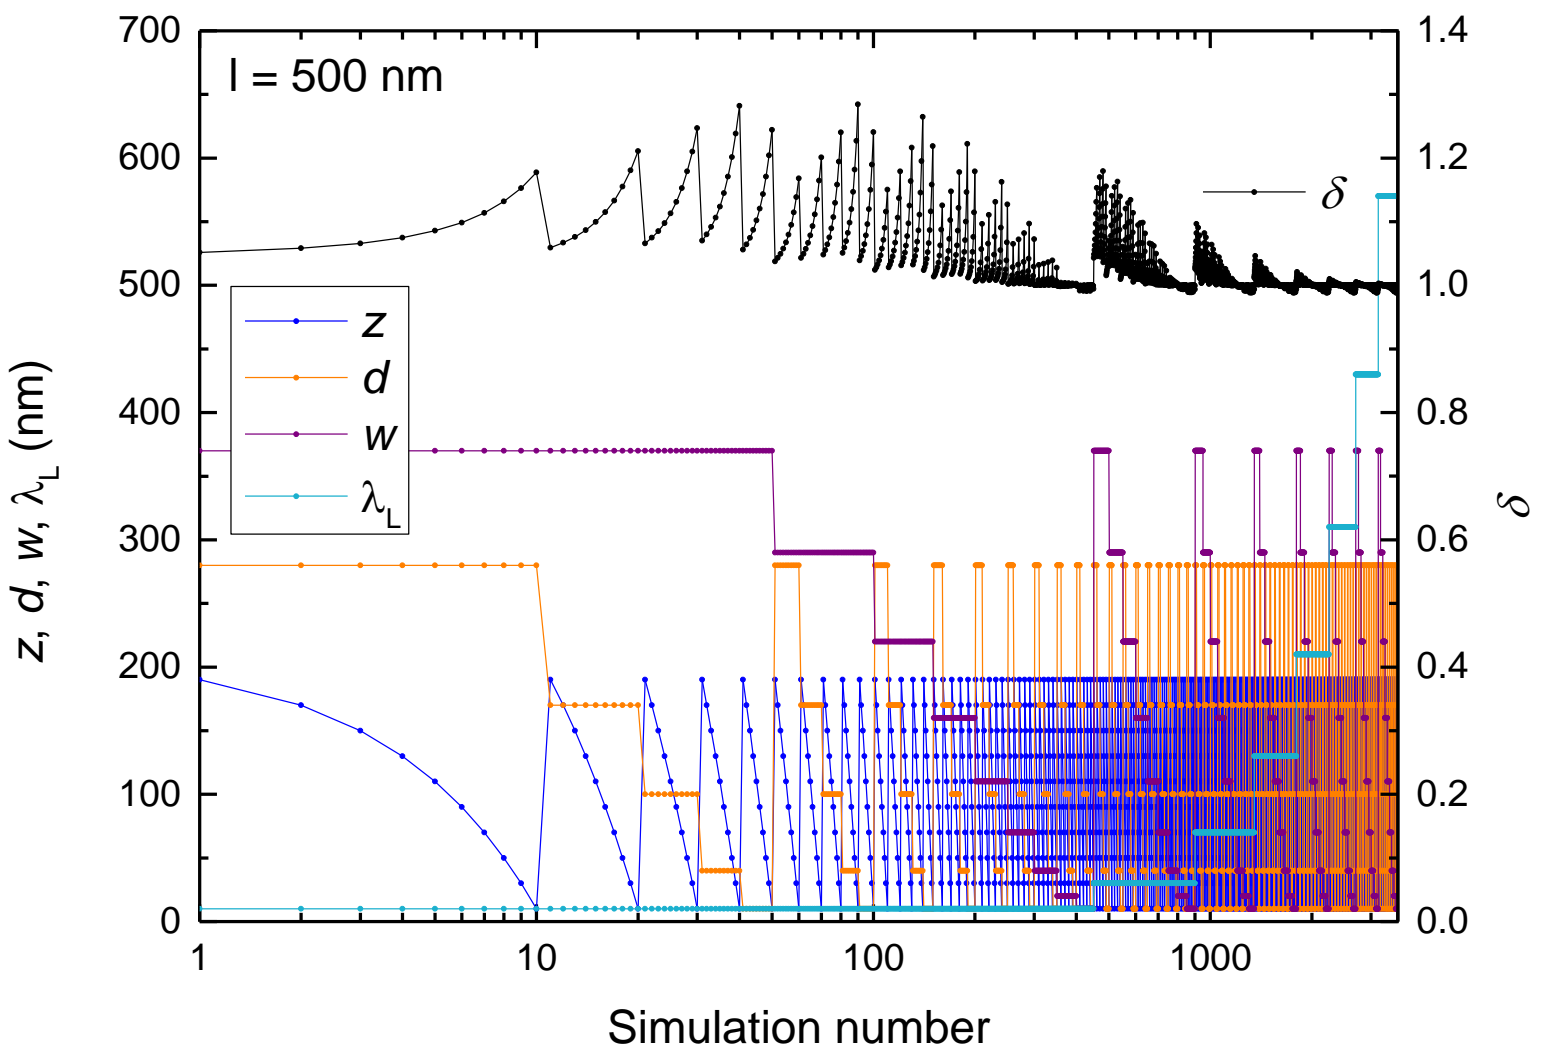

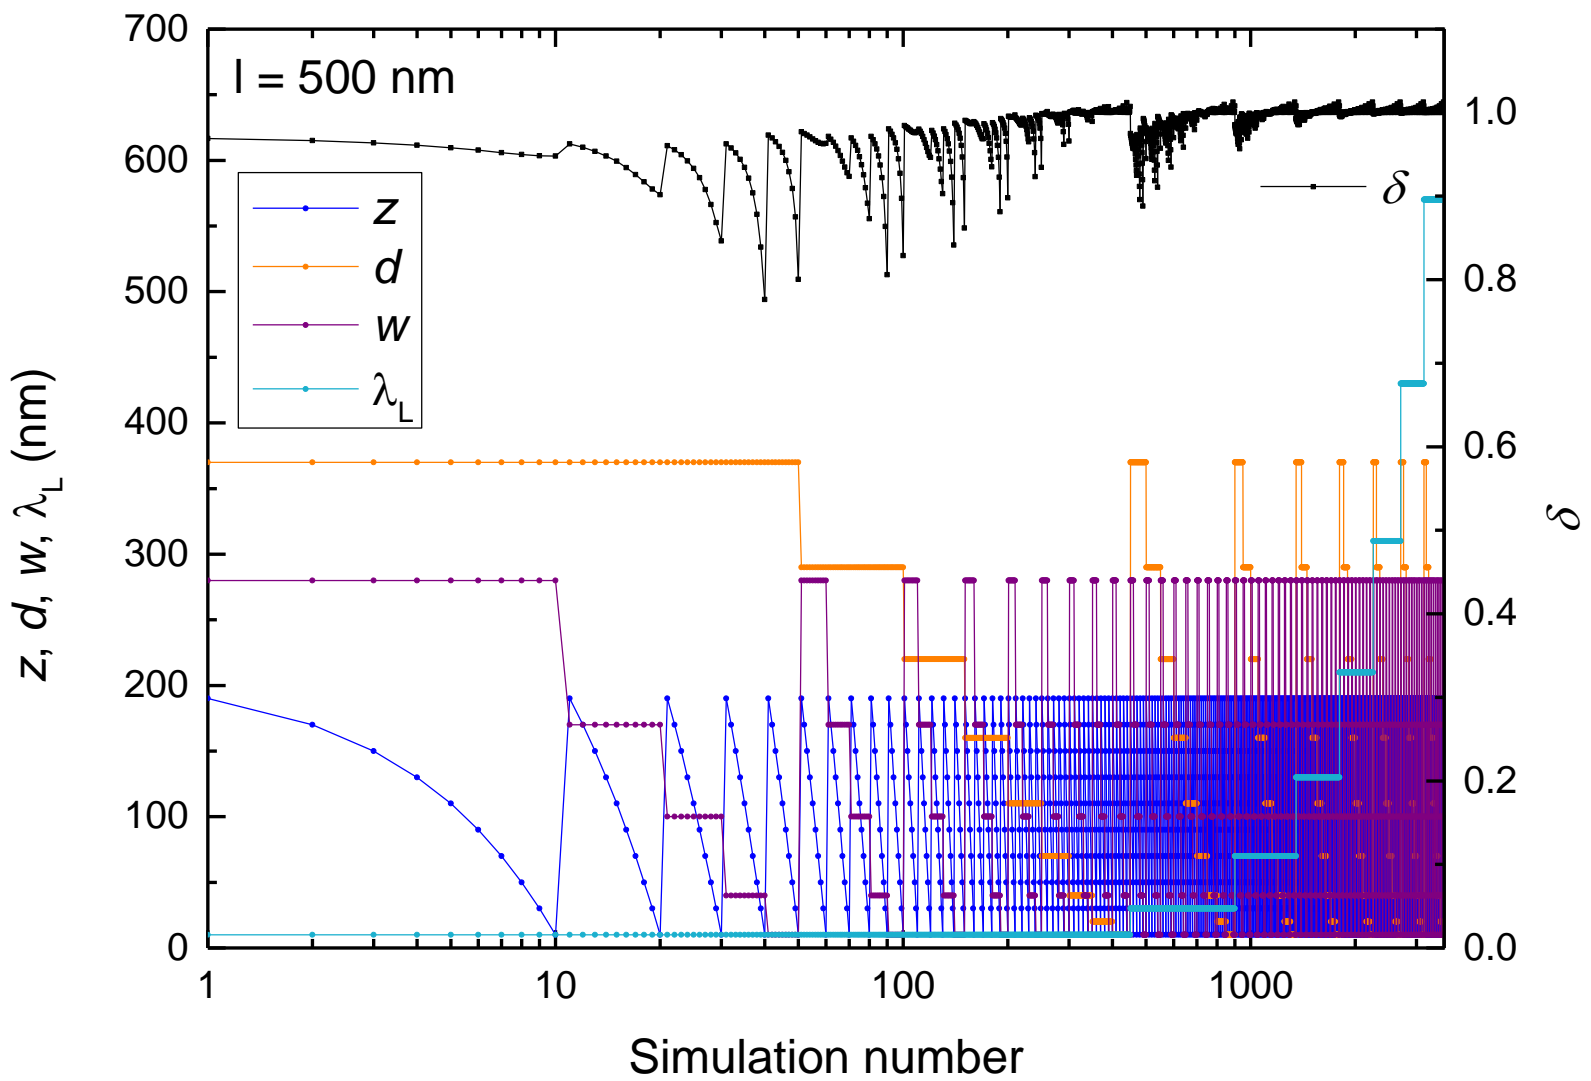



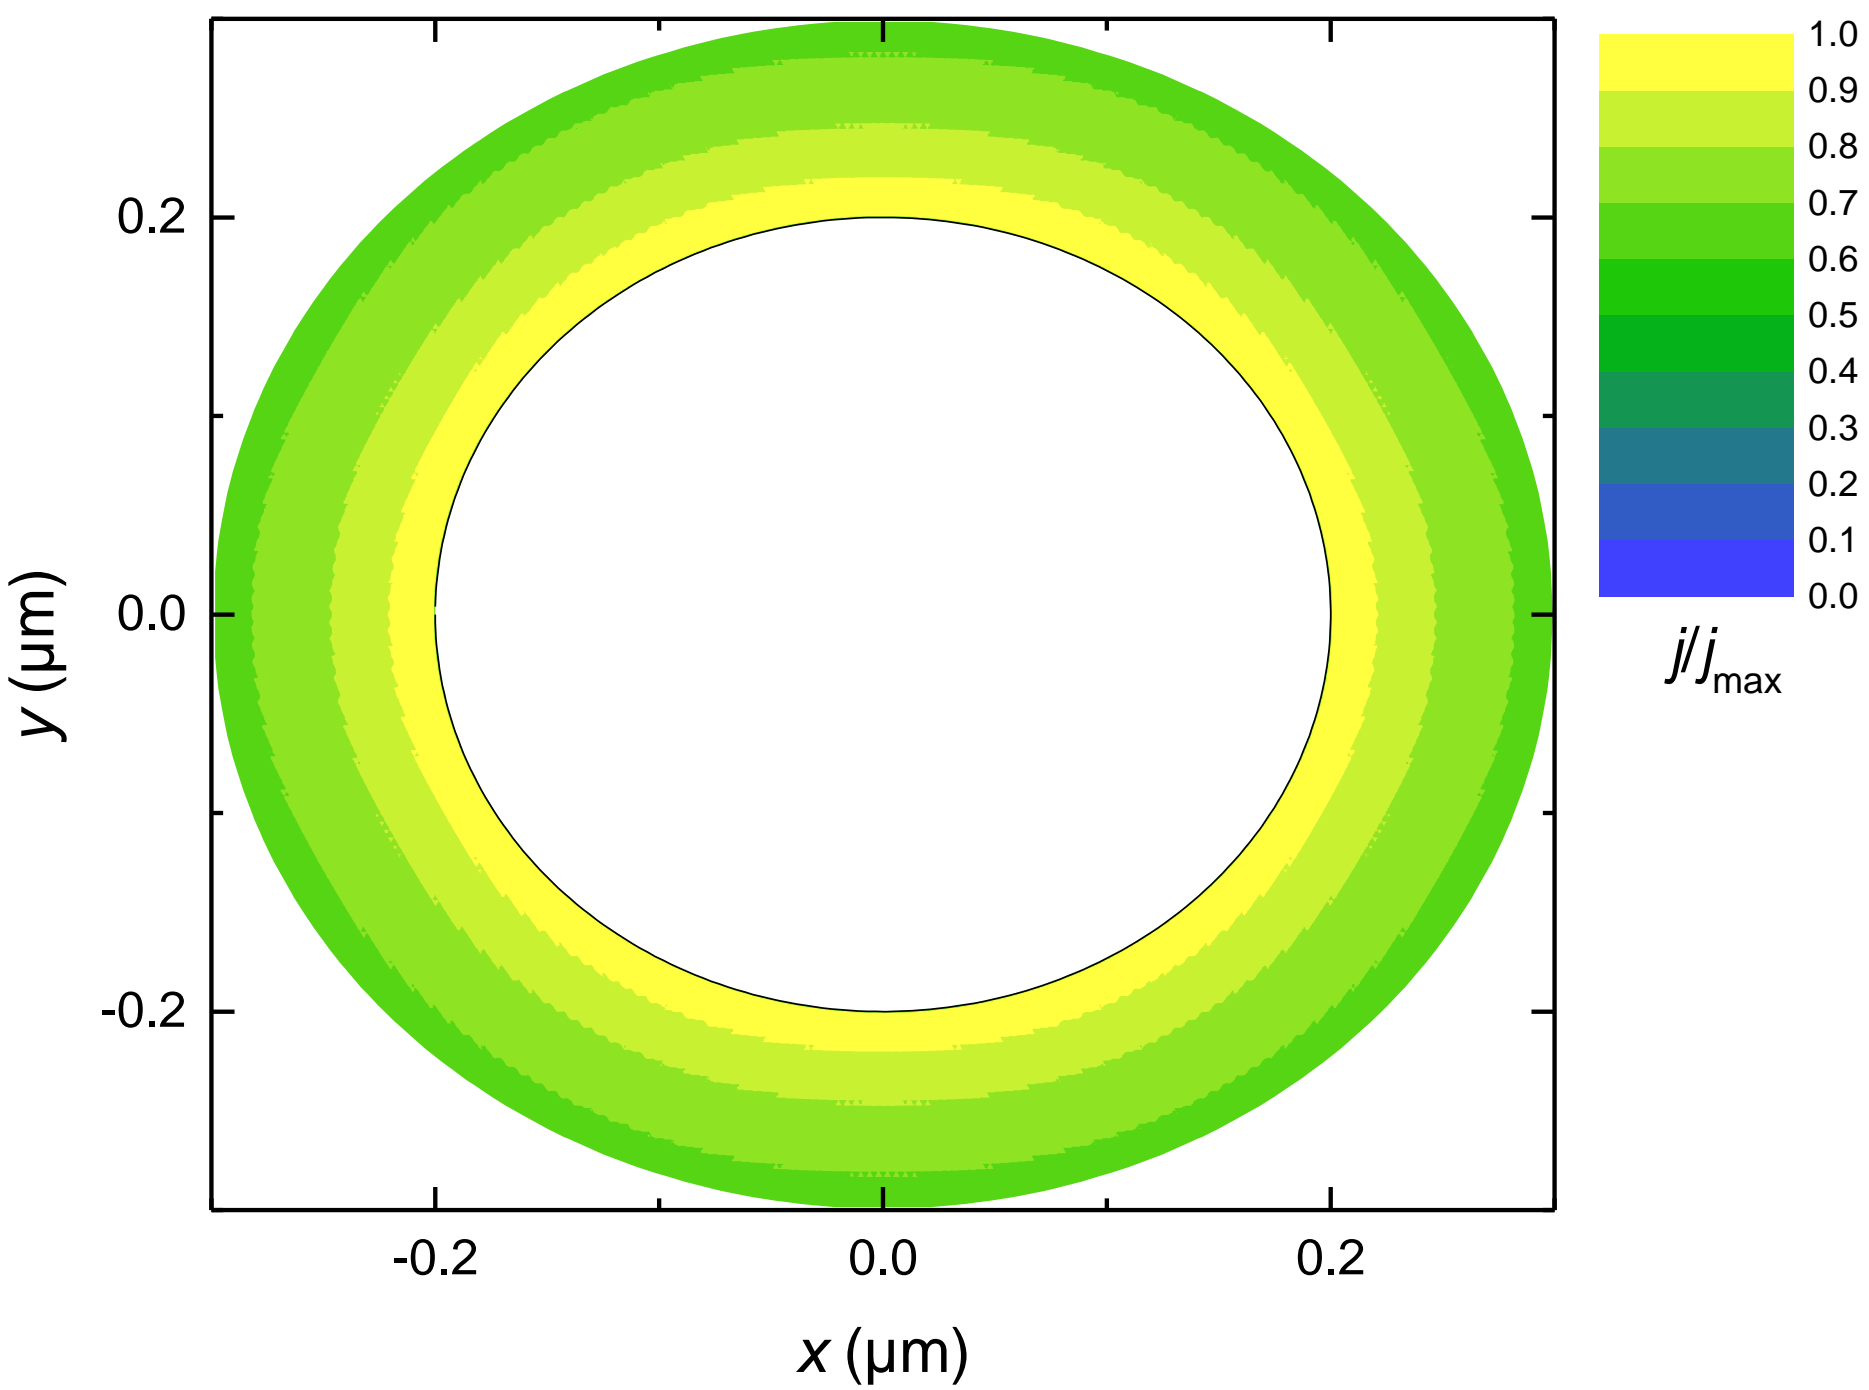

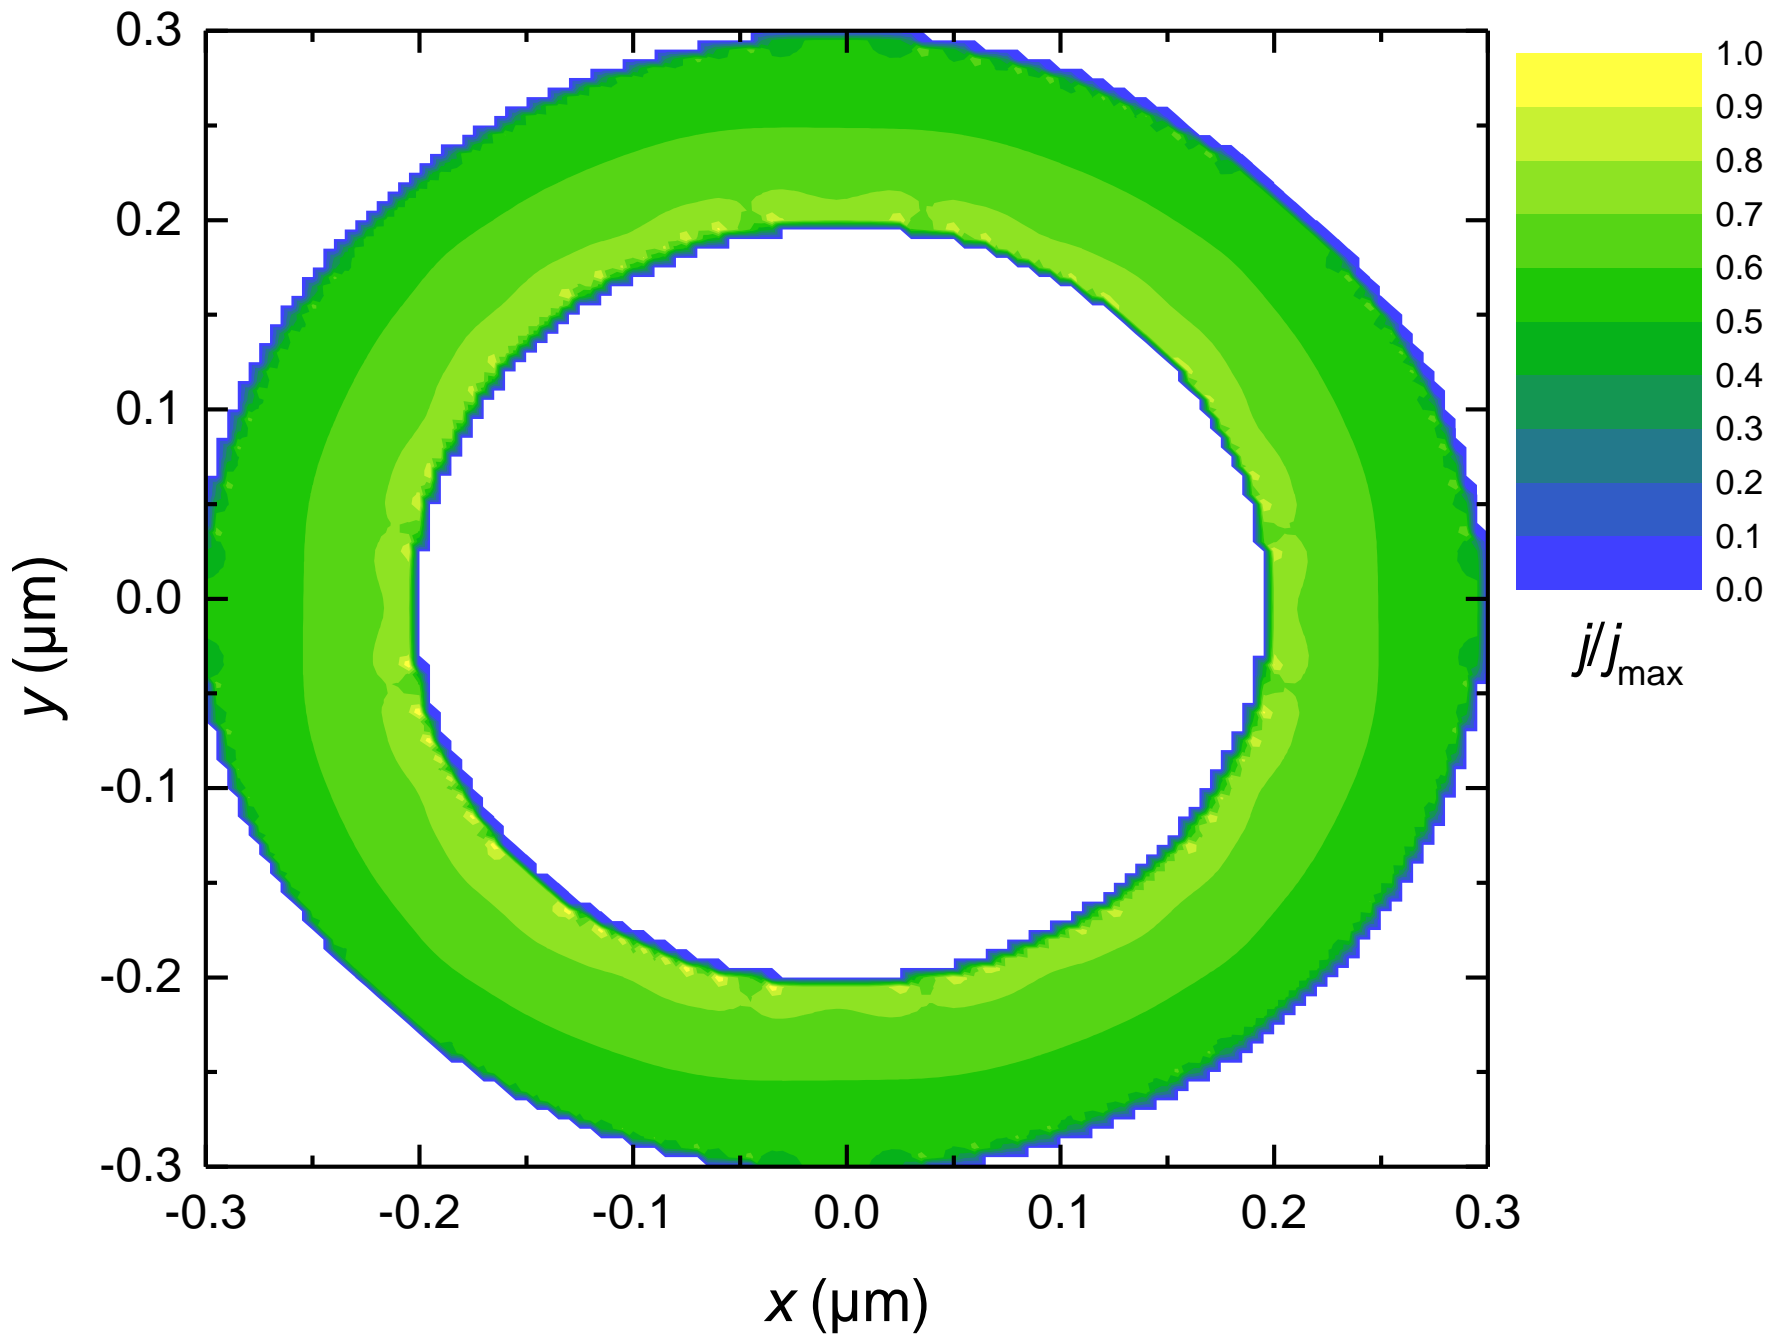

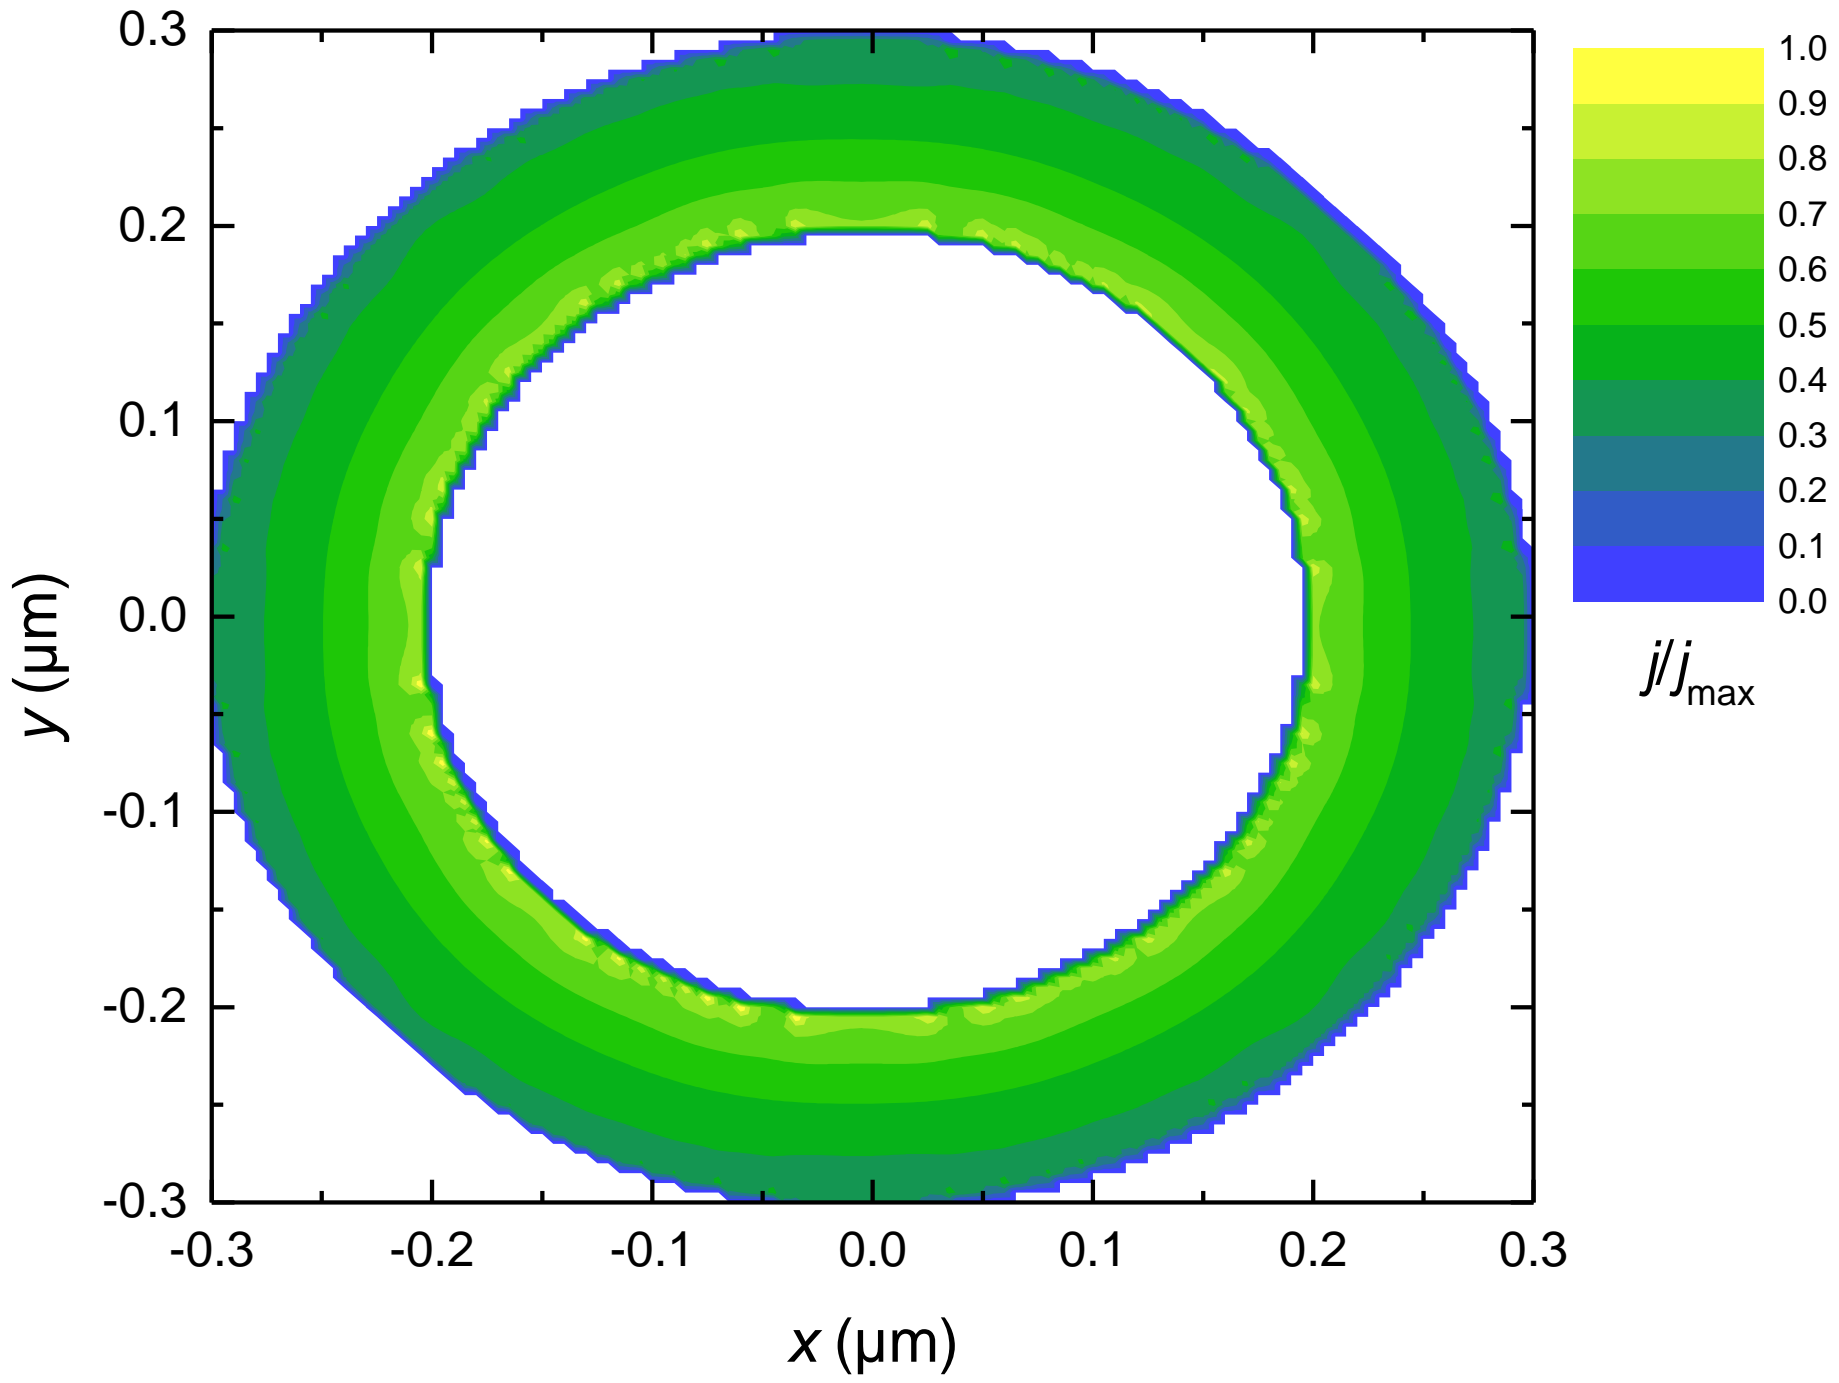

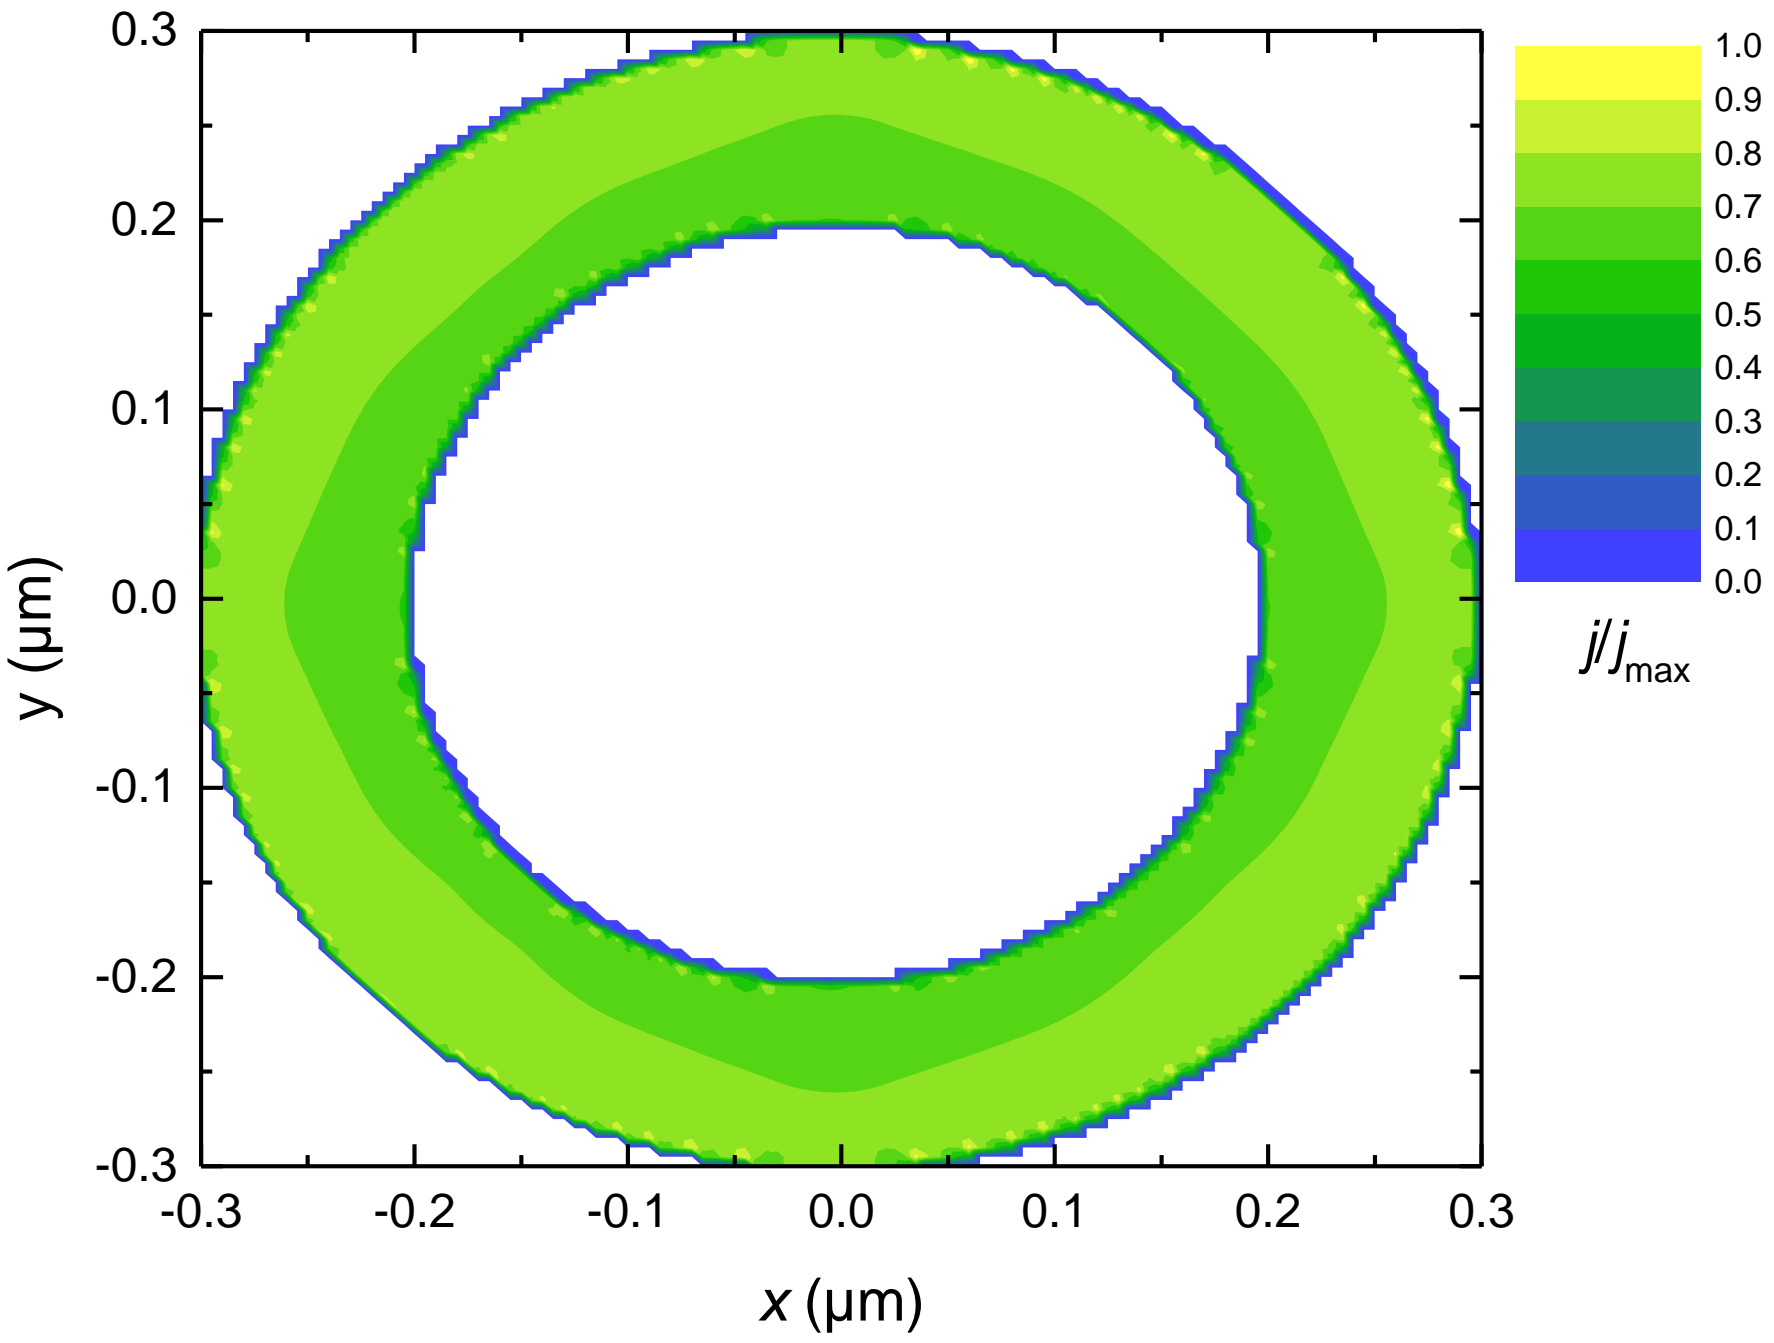

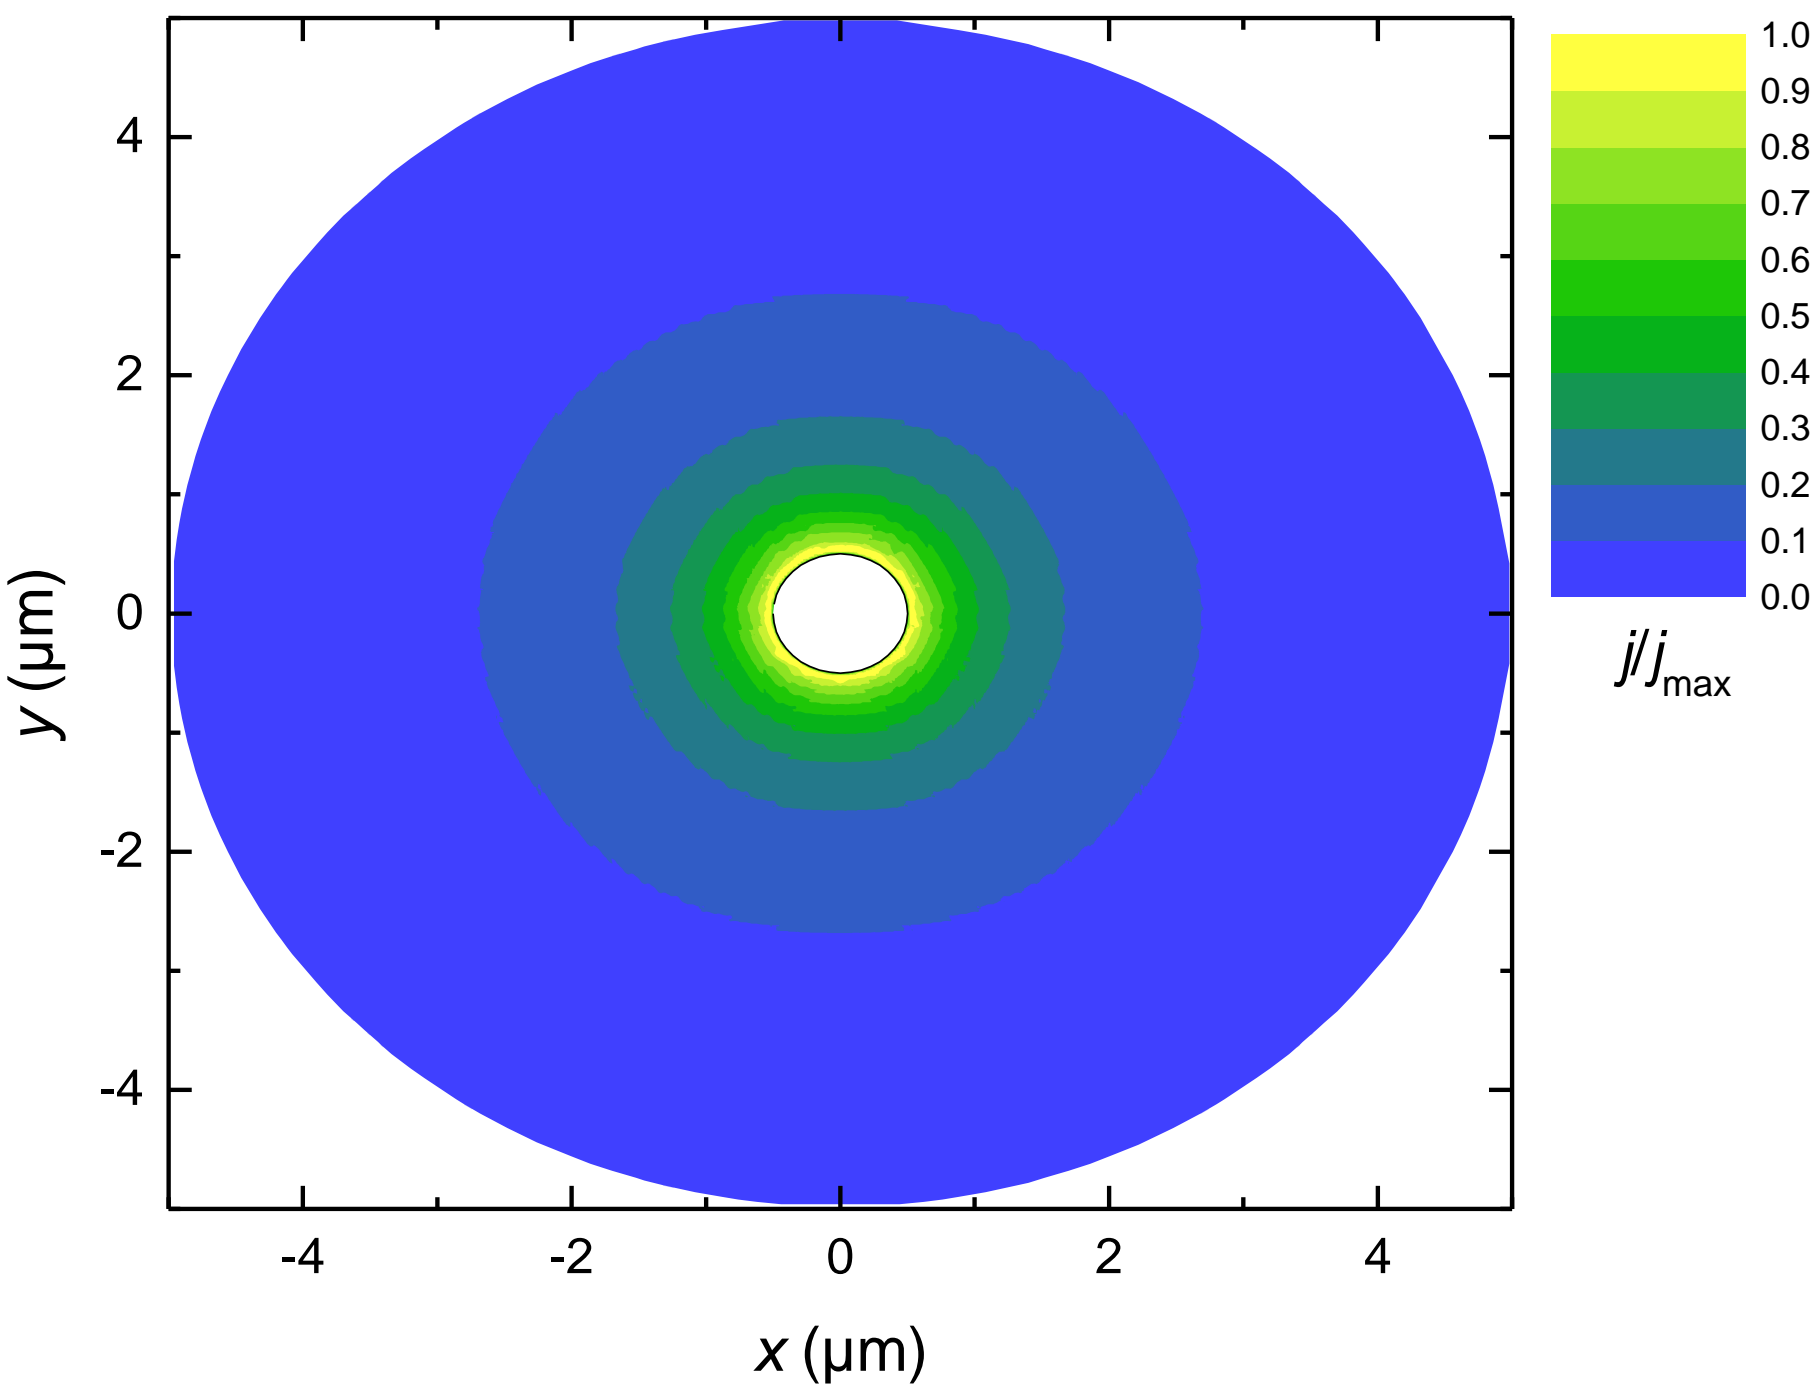

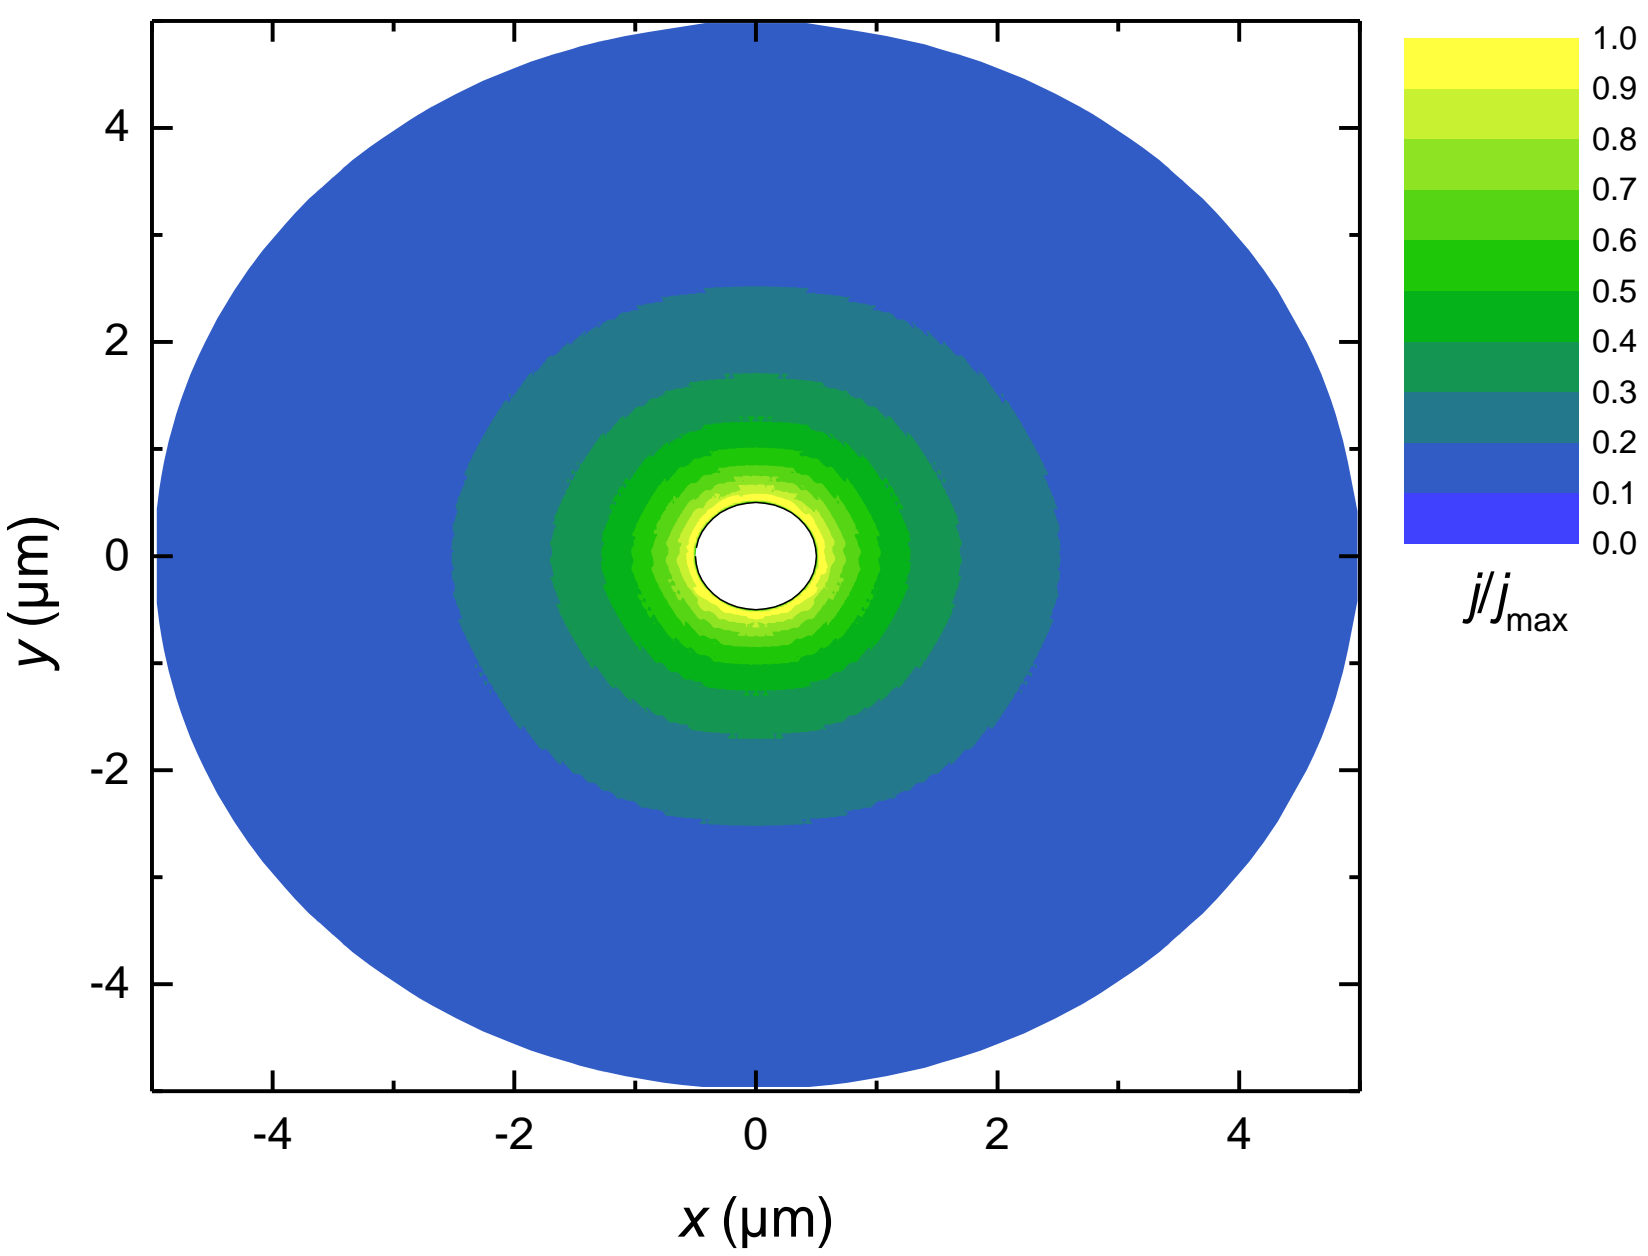

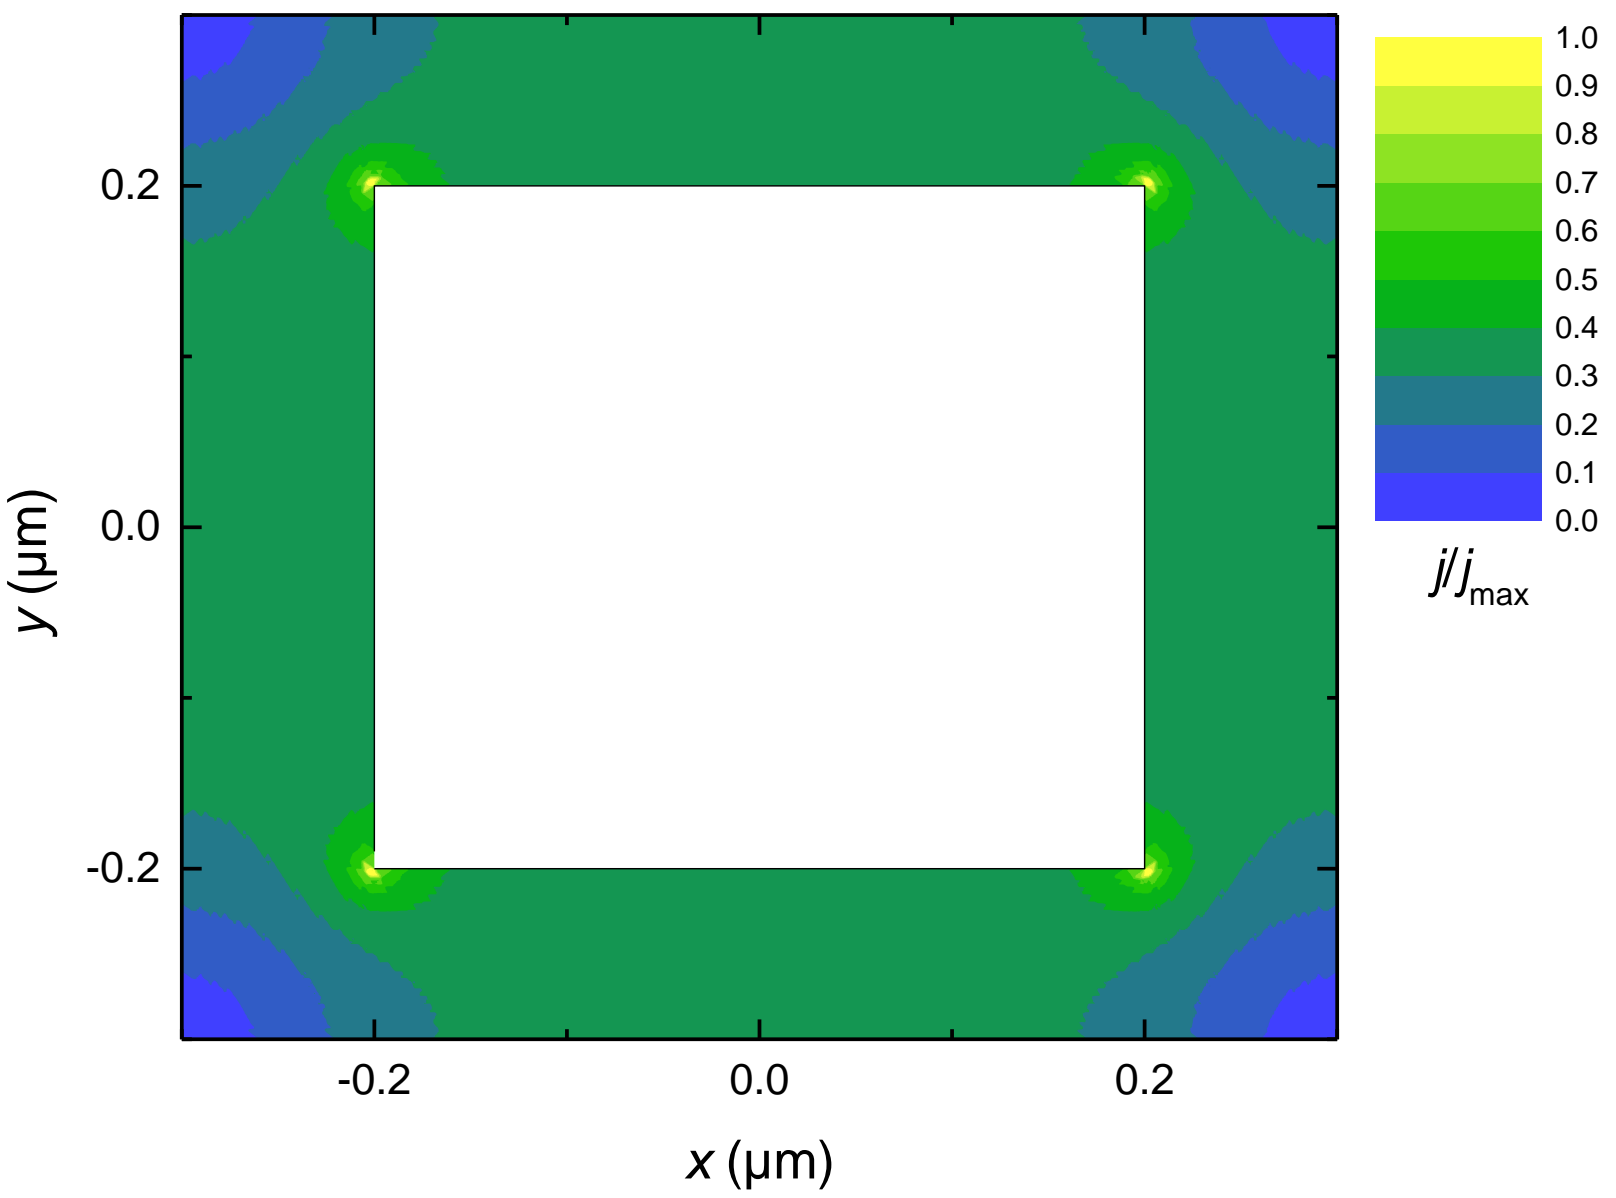

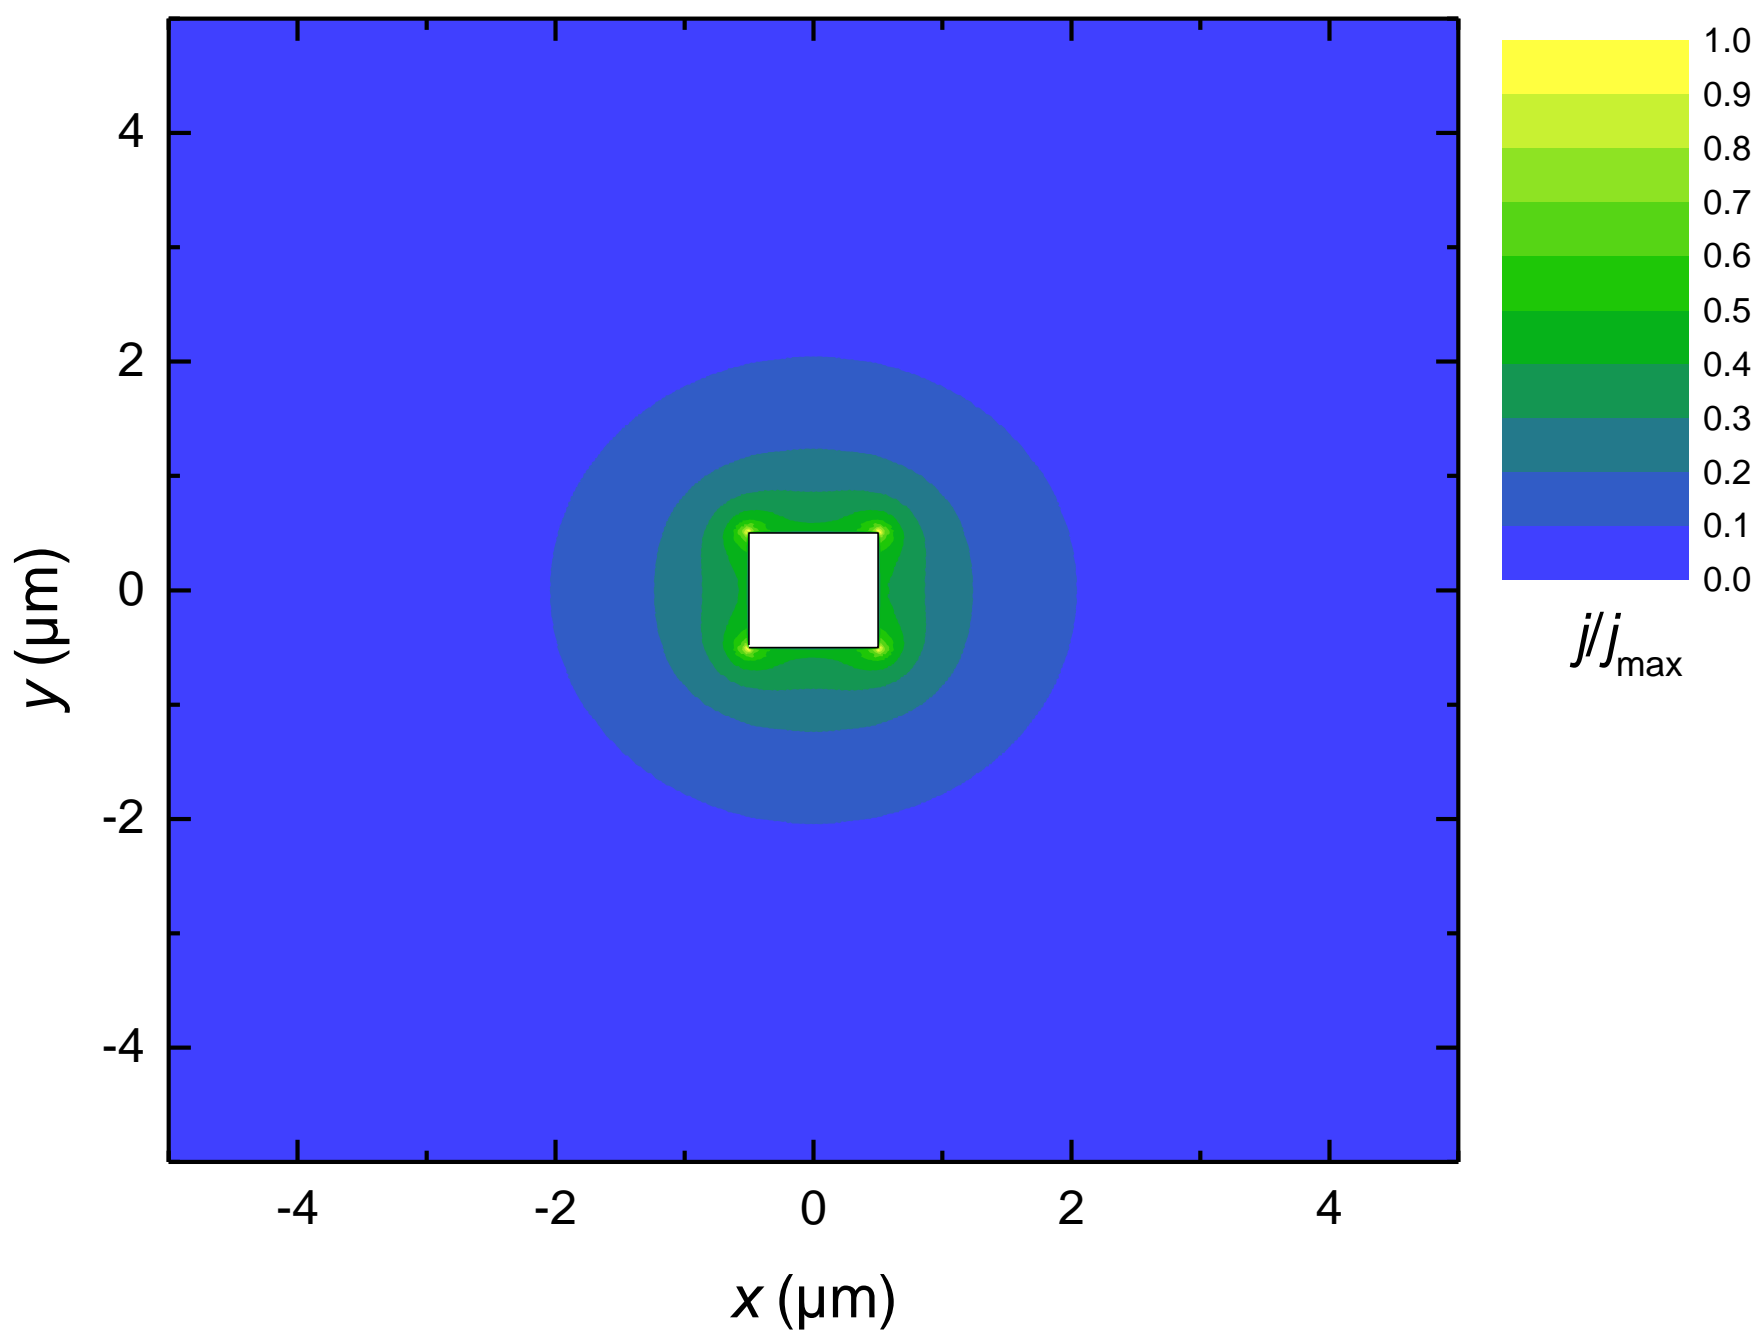



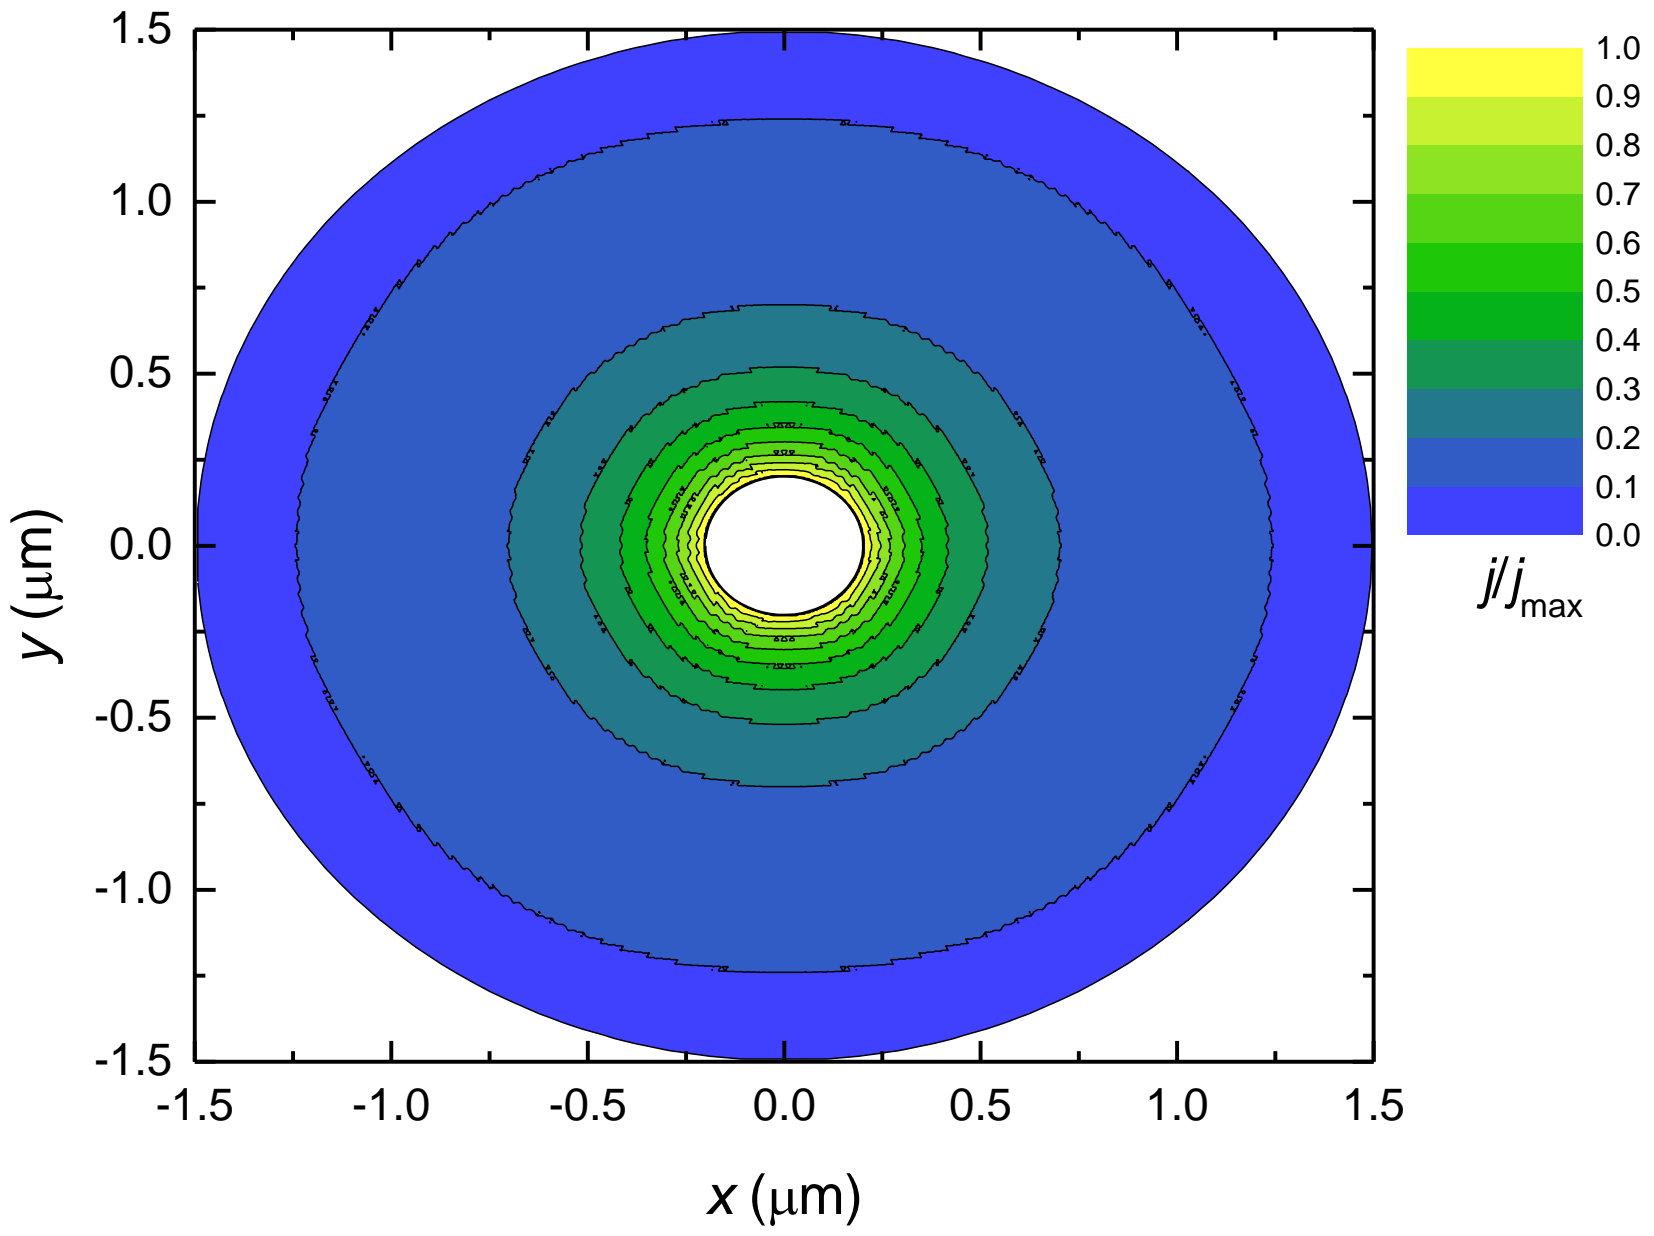

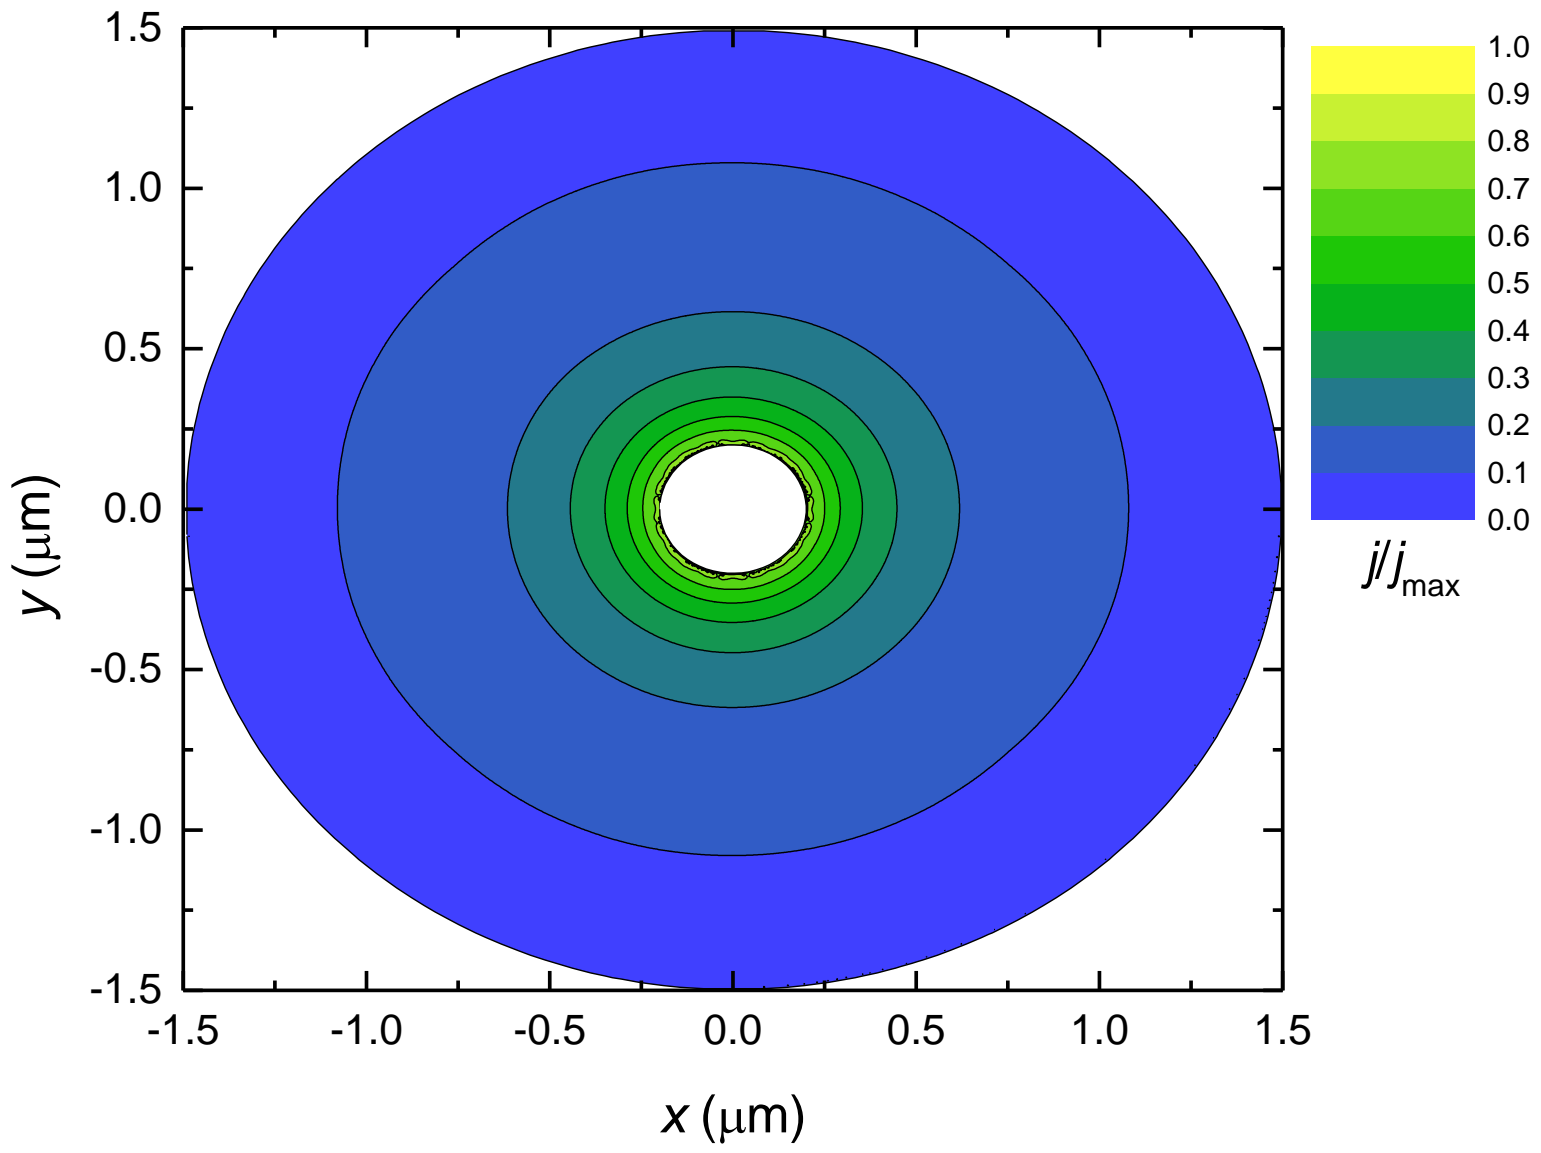

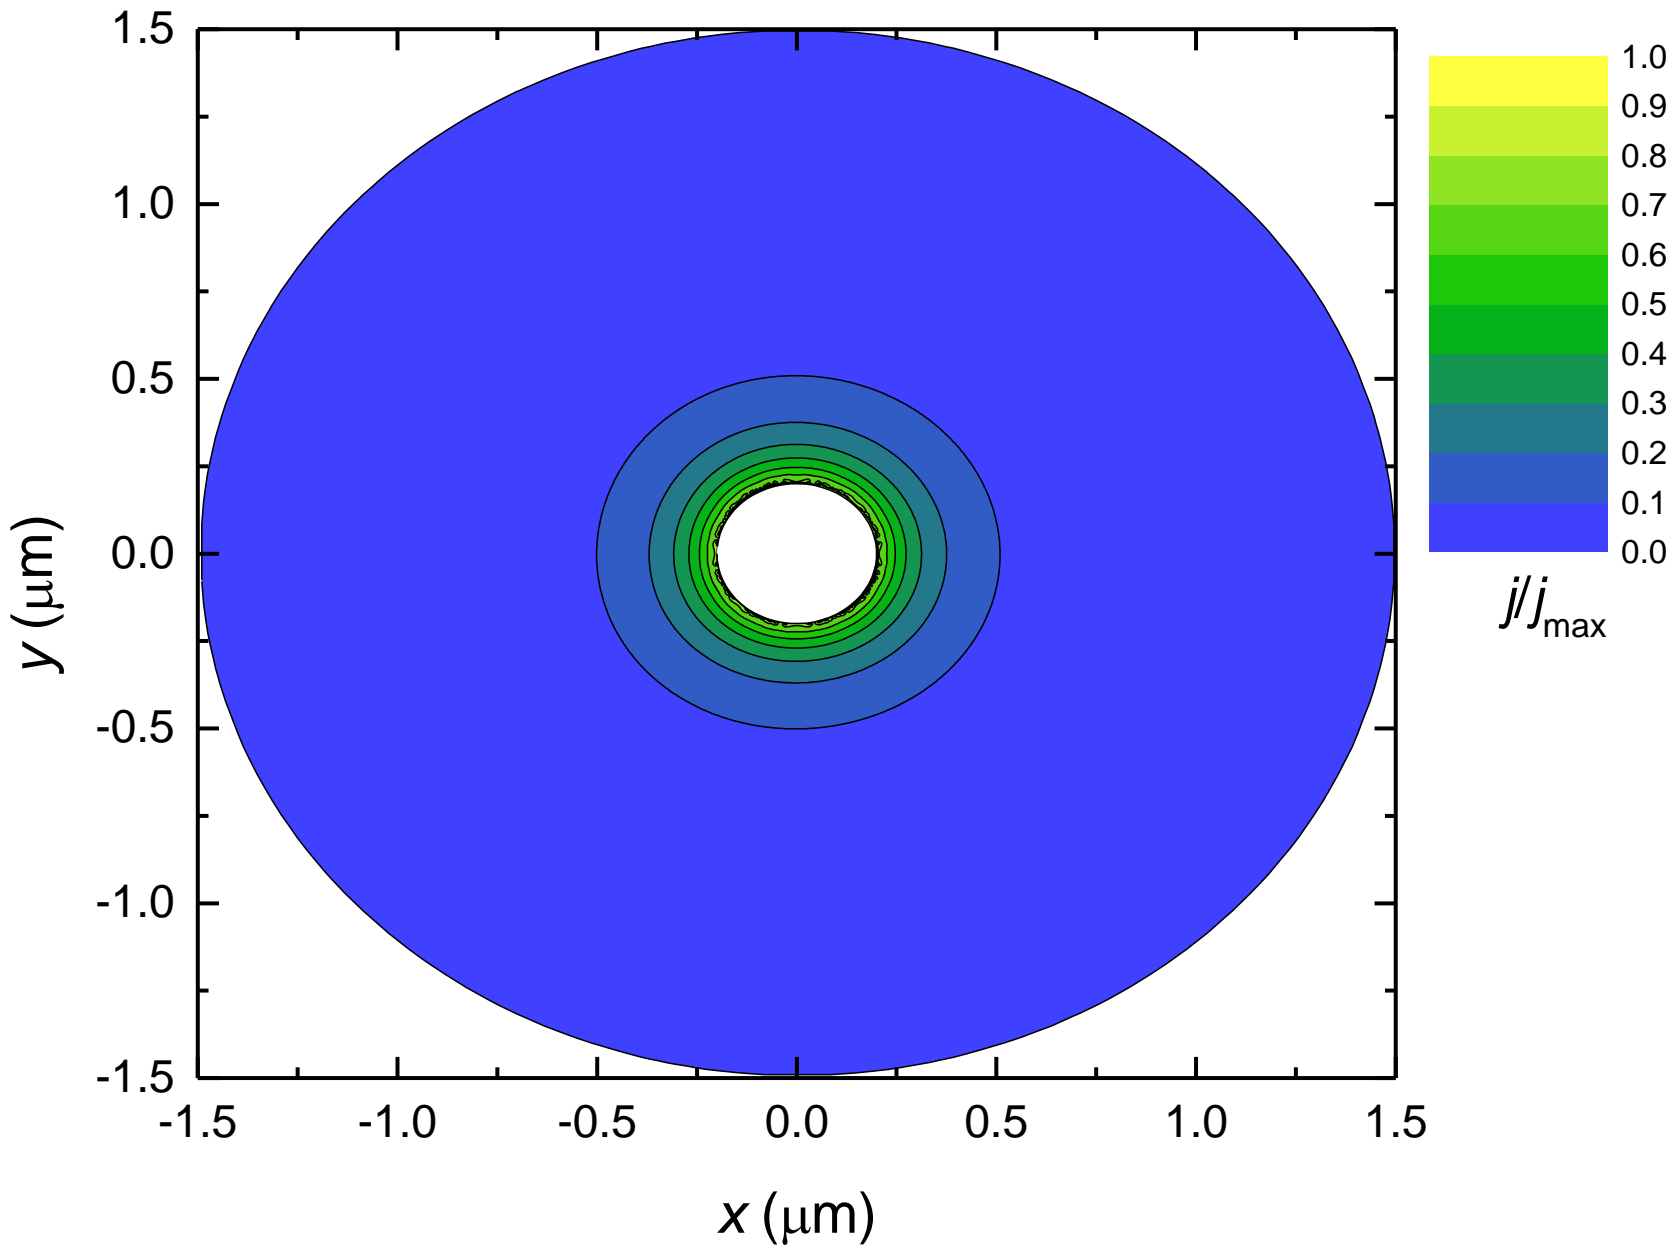

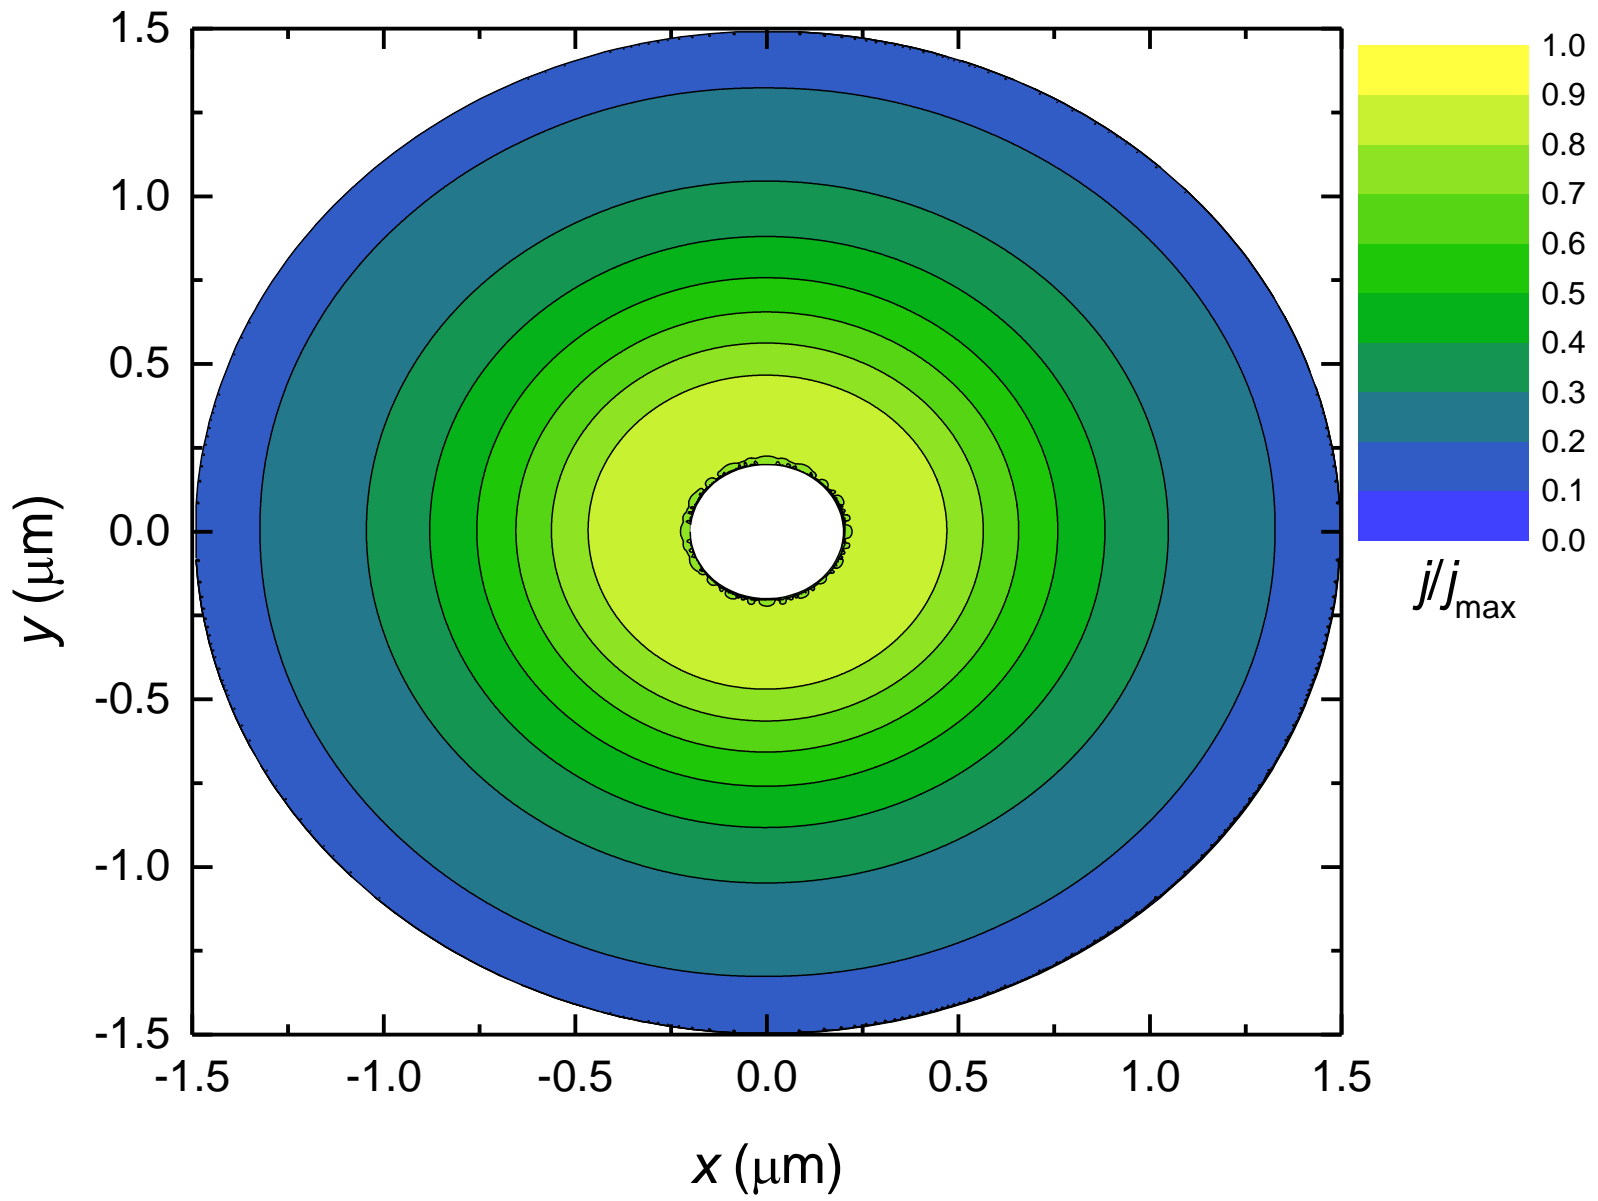

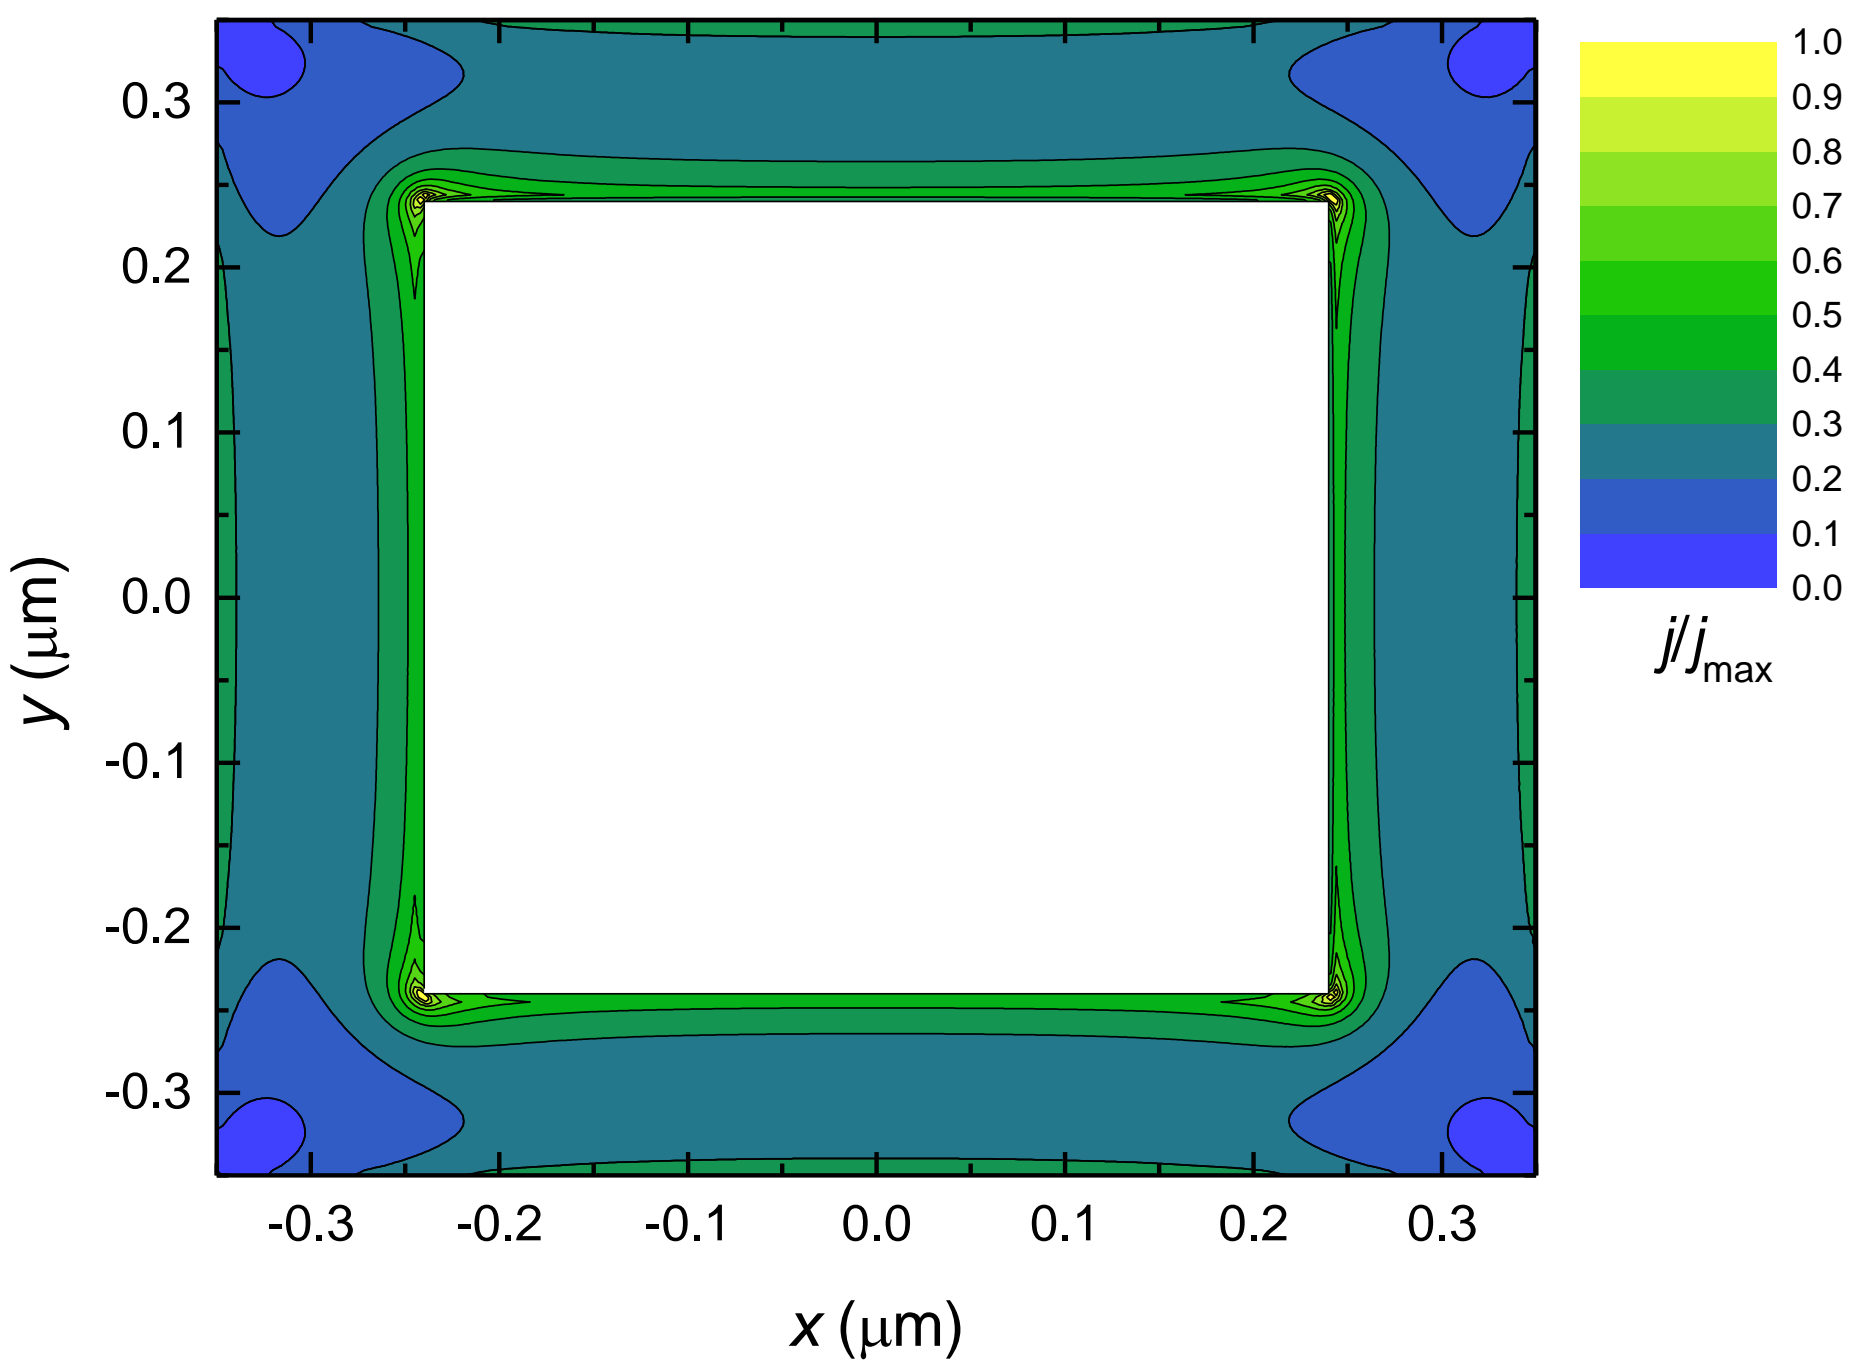

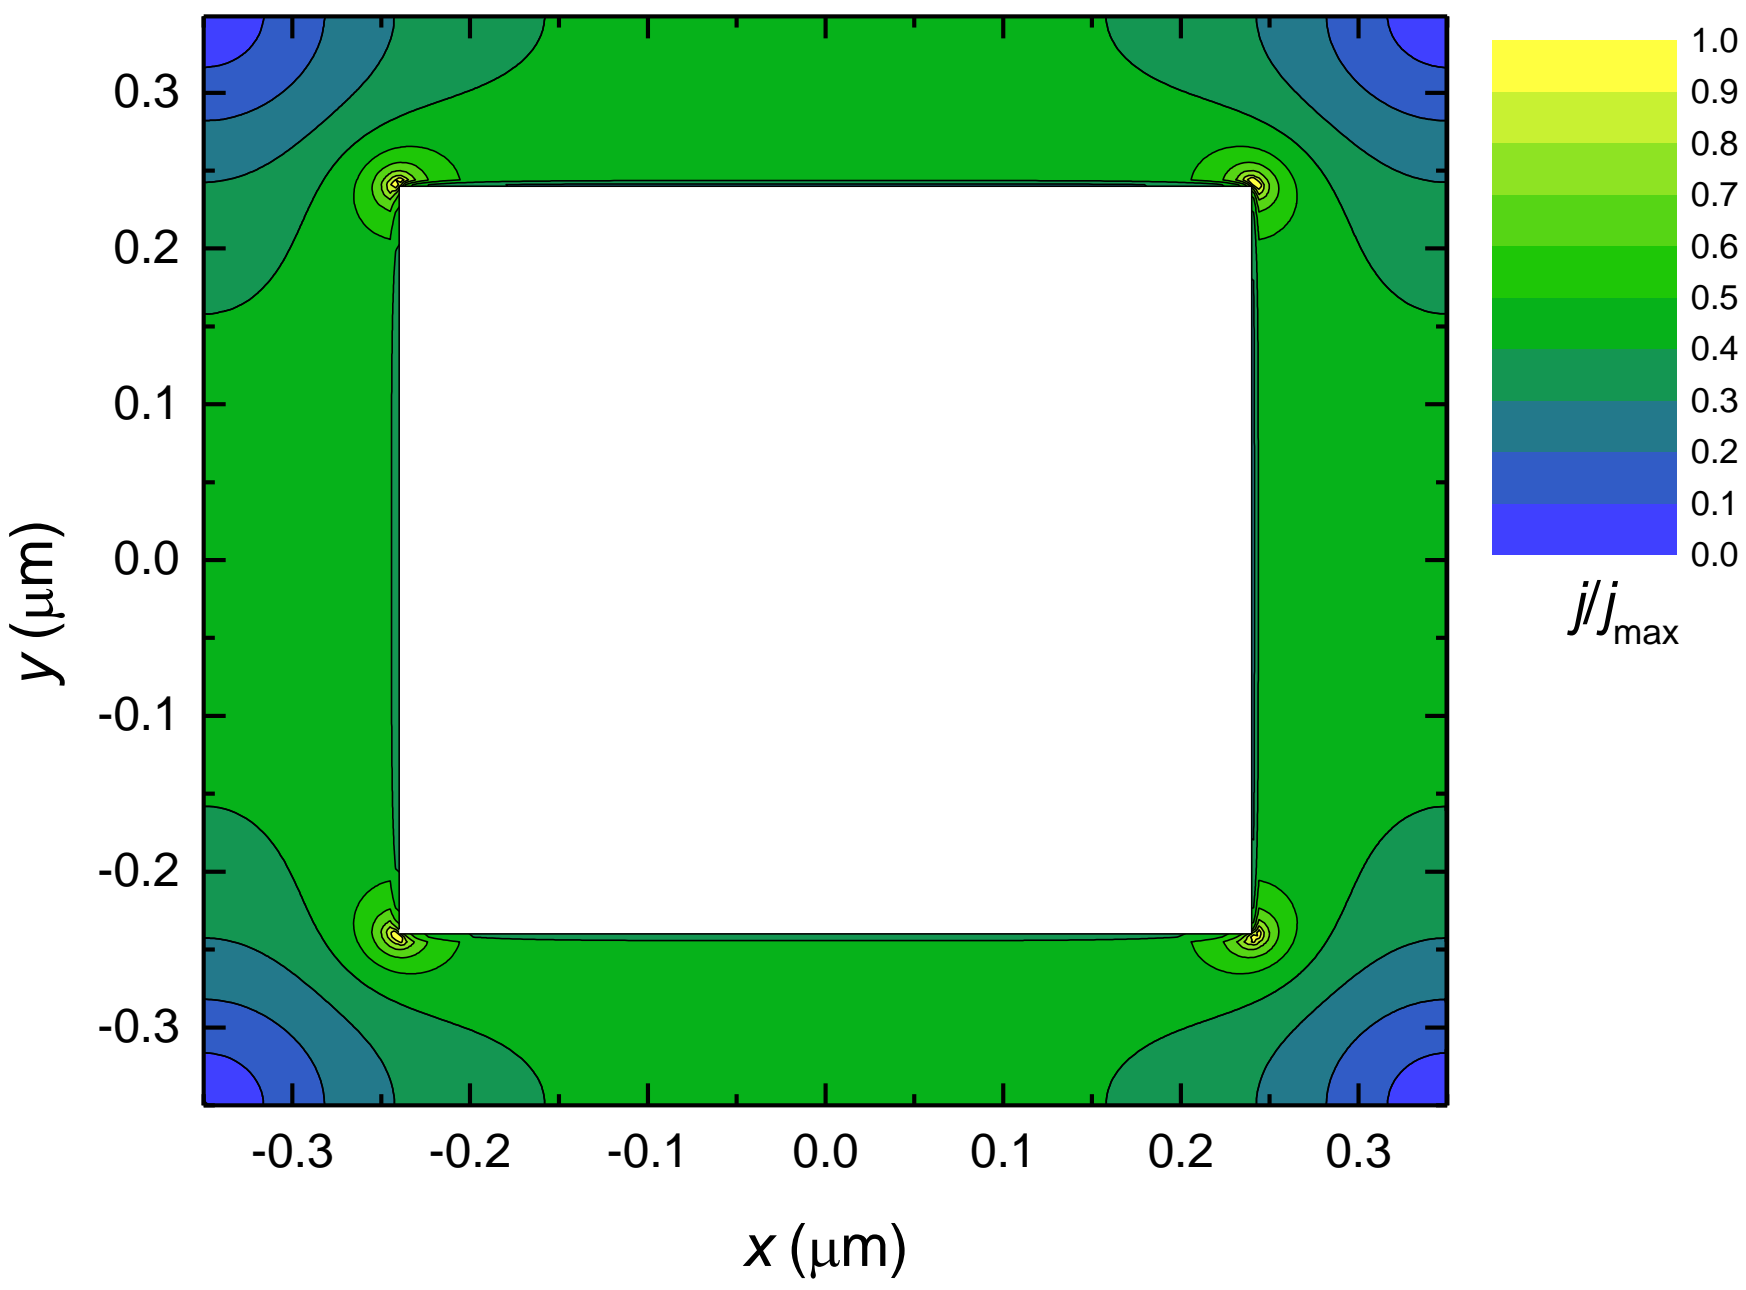

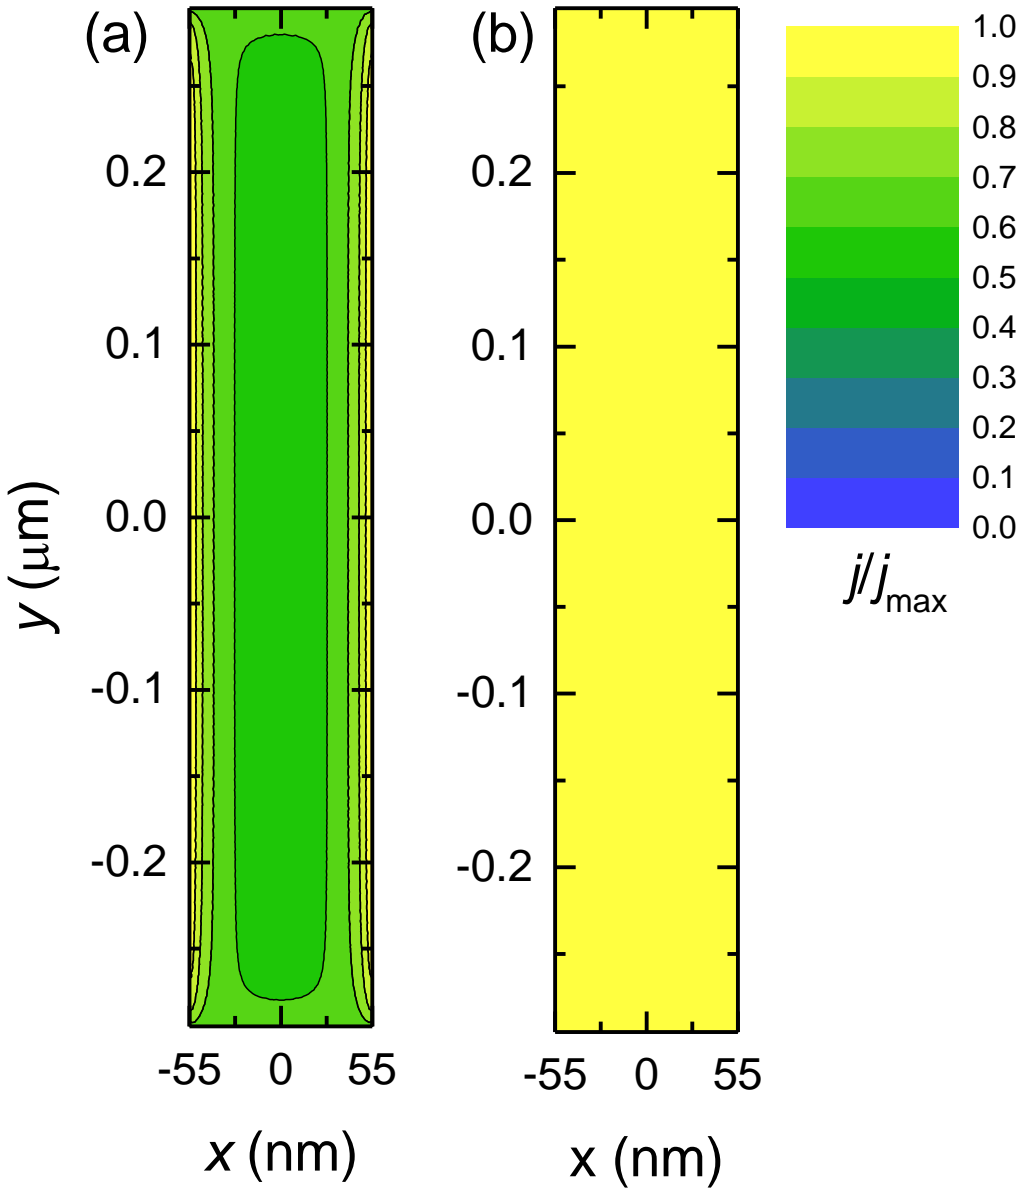

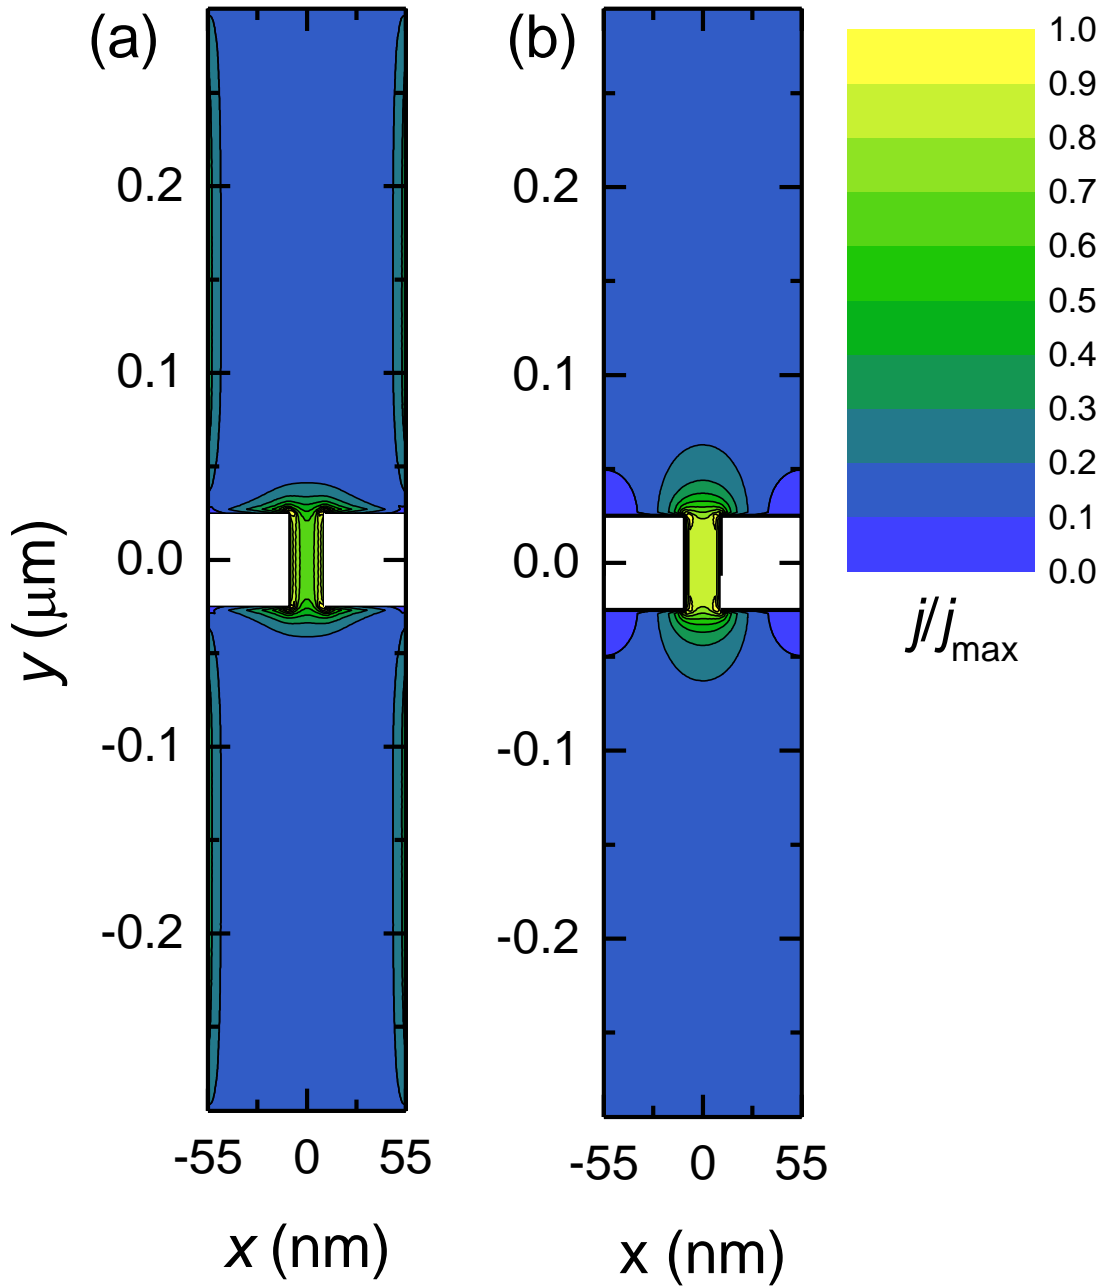

Supplement: Supplementary file 2 [file fig_supplement.pdf]
